# Supplementary material for: Hypothesis Testing for Two Sample Comparison of Network Data
Source: arXiv:2106.13931 source file (2021-06-26)
Supplement: Supplementary file 1 [file networktest_supp.pdf]

# Supplemental Materials for “Hypothesis Testing for Two Sample Comparison of Network Data”

Han Feng, Xing Qiu, Hongyu Miao

## S1 Universal Asymptotic Moment Properties of the Proposed Network Test

In this section, we provide a detailed proof of Theorem 2 in the main text, which is the main theoretical results we obtained for the proposed network test. Also included are a few small simulations to demonstrate the complexity of the asymptotic mean and covariance structure of the pairwise distance matrix and the  $F$ -statistic used in the proposed test.

### S1.1 A General Model for the Distance Matrix

Due to the space limit, only an outline of the theoretical investigations of the proposed network test is presented in the main text, Section 3. In this Supplementary text, we strive for a relatively long and rigorous derivation of the main results.

First, we describe a general model for the distance matrix and make some sweeping assumptions to facilitate large sample analyses.

1. **Two-group comparison:** Let  $\mathcal{G}_{n:1}^Z, \dots, \mathcal{G}_{n:n}^Z$ , for  $n = 1, 2, \dots$  be a triangular array of networks in which each row is a sample of  $n$  networks that can be divided into groups  $A$  and  $B$ , each with sample size  $n_A$  and  $n_B$  (therefore  $n = n_A + n_B$ ). WLOG, we may assume that each row is ordered so that the first  $n_A$  samples are from group  $A$ , and the rest  $n_B$  samples are from group  $B$ . When there is no confusion (as in the main text), we may drop the first  $n$  in  $\mathcal{G}_{n:i}^Z$ , which represents the sample size in large-sample analysis.
2. **Independence of observations:** All  $\mathcal{G}_{n:i}^Z$  within each row are assumed to be independent. Within each group, they are identically distributed:

$$\mathcal{G}_{n:i}^Z \sim \begin{cases} P_A, & i \in A, \\ P_B, & i \in B. \end{cases} \quad (\text{S.1})$$

3. **Equal distribution under the null:** Under  $H_0$ , groups  $A$  and  $B$  share the same distribution function:  $P_A = P_B$ . In this case, we will denote both  $P_A$  and  $P_B$  as  $P_0$ . Under  $H_1$ , these two distributions are assumed to be different.
4. **Axioms of the distance function:** There is a distance function  $d(\cdot, \cdot)$  defined for those networks that satisfies the three axioms for distance: (a)  $d(x, y) = 0$  iff  $x = y$ , (b)  $d(x, y) = d(y, x)$ , and (c)  $d(x, y) \leq d(x, z) + d(z, y)$ . We will use  $\mathcal{D}_n$  as a notation for the  $n \times n$ -dimensional squared pairwise distance matrix between all samples in the  $n$ th row of the triangular array, i.e.,  $\mathcal{D}_{n,i,j} = d^2(\mathcal{G}_{n:i}^Z, \mathcal{G}_{n:j}^Z)$ . When there is no confusion, we may drop the subscript “ $n$ ” from  $\mathcal{D}_n$ .

5. **Symmetry of within-groups distance:** By construction,  $\mathcal{D}_n$  is a symmetric matrix with zero diagonal elements. Based on the within-group *i.i.d.* assumption, we know that the marginal distribution of  $\mathcal{D}_{n,ij}$  can only take three forms for  $i \neq j$

$$\mathcal{D}_{n,ij} \sim \begin{cases} g_A(x), & i, j \in A, \\ g_B(x), & i, j \in B, \\ g_{\text{between}}(x), & i \in A, j \in B, \text{ or } i \in B, j \in A. \end{cases} \quad (\text{S.2})$$

We further assume that group labels  $A$  and  $B$  are symmetric in marginal distributions:  $g_A(x) = g_B(x) = g_{\text{within}}(x)$  so that the main focus of the two-group comparison is based on the differences between  $g_{\text{within}}(x)$  and  $g_{\text{between}}(x)$ .

6. **Finite moments:** When viewed as a random matrix,  $\mathcal{D}_n$  has finite first and second order moments.

As a remark, the first three assumptions are given in Section 2.2 of the main text (albeit in less elaborated form); the 4th assumption is implied by the fact that our proposed method is based on a distance matrix, and the last two assumptions are specified in Section 3.1 in the main text.

## S1.2 Representation of the Mean and Covariance of $\mathcal{D}$

With the assumptions made in Section S1.1, we can represent the expectation of  $\mathcal{D}$  as

$$E(\mathcal{D}_{ij}) = \begin{cases} 0, & i = j. \\ \mu_{\text{within}}, & i, j \in A \text{ or } i, j \in B, i \neq j. \\ \mu_{\text{between}} := \mu_{\text{within}} + \delta_\mu, & i \in A, j \in B, \text{ or } i \in B, j \in A. \end{cases} \quad \begin{cases} \delta_\mu = 0, & \text{under } H_0 \\ \delta_\mu > 0, & \text{under } H_1. \end{cases} \quad (\text{S.3})$$

Let  $\mathbf{1}_n \in \mathbb{R}^n$  be a vector containing all ones,  $J_n = \mathbf{1}_n \mathbf{1}_n'$  be an  $n \times n$ -dimensional matrix with all ones. Let  $\mathbf{1}_A \in \mathbb{R}^n$  be the binary vector that represents group  $A$ , namely,  $1_{A,i}$ , the  $i$ th element in  $\mathbf{1}_A$ , equals one if the  $i$ th network is from group  $A$  and zero if it is from group  $B$ . Consequently,  $\mathbf{1}_B := \mathbf{1}_n - \mathbf{1}_A$  is a binary vector that represents group  $B$ .

We can re-write Equation (S.3) in matrix notation as

$$E(\mathcal{D}) = \mu_{\text{within}}(J_n - I_n) + \delta_\mu (\mathbf{1}_A \mathbf{1}_B' + \mathbf{1}_B \mathbf{1}_A'). \quad (\text{S.4})$$

Next, we will work on the covariance  $\text{cov}(\mathcal{D}_{ij}, \mathcal{D}_{i'j'})$ . For simplicity, we denote  $\Sigma := \Sigma(\text{vec}(\mathcal{D}))$ .

Since  $\mathcal{D}$  is a pairwise distance matrix,  $\mathcal{D}_{ii} = 0$  for  $i = 1, 2, \dots, n$ , so  $\text{cov}(\mathcal{D}_{ij}, \mathcal{D}_{i'j'}) = 0$  if either  $i = j$  or  $i' = j'$ . Therefore, we will focus on other cases ( $i \neq j$  and  $i' \neq j'$ ). Due to the independence assumption,  $\text{cov}(\mathcal{D}_{ij}, \mathcal{D}_{i'j'}) = 0$  if  $i, j, i', j'$  are all distinct, so we can assume that at least two of these four indices are identical. Due to the symmetry of groups assumption and the intrinsic symmetry of distance (*i.e.*,  $\mathcal{D}_{ij} = \mathcal{D}_{ji}$ ) and covariance ( $\text{cov}(\mathcal{D}_{ij}, \mathcal{D}_{i'j'}) = \text{cov}(\mathcal{D}_{i'j'}, \mathcal{D}_{ij})$ ), we only need to consider five different cases for  $(E(\mathcal{D}_{ij}), E(\mathcal{D}_{i'j'}), \Sigma_{ij,i'j'})$ . For simplicity, we will use simplified notation  $(A, B, A, B)$  to represent the membership of  $(i, i', j, j')$ . Note that the symmetry of groups assumption implies that  $\text{cov}(\mathcal{D}_{ij}, \mathcal{D}_{i'j'})$  is preserved if we simultaneously swap the group labels of all four indices  $(i, j, i', j')$  from one group to another, e.g.,  $(A, B, B, A) \rightarrow (B, A, A, B)$ .

Below we list these five cases. Note that in all those cases, we assume that  $i \neq j, i' \neq j'$ . Main cases (those with size  $m_k = O(n^3)$ ) are highlighted in bold face.

Case 1:  $AAAA$  or  $BBBB$ ;  $i = i', j = j'$ , or  $i = j', i' = j$ .  $E(\mathcal{D}_{ij}) = E(\mathcal{D}_{i'j'}) = \mu_{\text{within}}$ .  $\Sigma_{ij,i'j'} = \sigma_1^2$ . The size (number of combinations) of this case is

$$m_1 = 2n_A(n_A - 1) + 2n_B(n_B - 1) = 2(n_A^2 + n_B^2) - 2n. \quad (\text{S.5})$$

**Case 2:**  $AAAA$  or  $BBBB$ ;  $(i = i', j \neq j')$ ,  $(i = j', i' \neq j)$ ,  $(i \neq j', j = i')$ , or  $(i \neq i', j = j')$ .  $E(\mathcal{D}_{ij}) = E(\mathcal{D}_{i'j'}) = \mu_{\text{within}}$ .  $\Sigma_{ij,i'j'} = \sigma_2^2$ . Its size is

$$\begin{aligned} \mathbf{m}_2 &= 4(n_A(n_A - 1)(n_A - 2) + n_B(n_B - 1)(n_B - 2)) \\ &= 4(n_A^3 + n_B^3 - 3(n_A^2 + n_B^2) + 2n). \end{aligned} \quad (\text{S.6})$$

**Case 3:**  $(AAAB, i = i' \text{ or } j = i')$ ,  $(AABA, i = j' \text{ or } j = j')$ ,  $(ABAA, i = i' \text{ or } i = j')$ ,  $(BAAA, j = i' \text{ or } j = j')$ .  $(E(\mathcal{D}_{ij}) = \mu_{\text{within}}, E(\mathcal{D}_{i'j'}) = \mu_{\text{between}})$  or  $(E(\mathcal{D}_{ij}) = \mu_{\text{between}}, E(\mathcal{D}_{i'j'}) = \mu_{\text{within}})$ .  $\Sigma_{ij,i'j'} = \sigma_2^2$ . Its size is

$$\mathbf{m}_3 = 8(n_A(n_A - 1)n_B + n_B(n_B - 1)n_A) = 8n_A n_B (n - 2). \quad (\text{S.7})$$

Case 4:  $(ABAB, i = i', j = j')$ ,  $(ABBA, i = j', j = i')$ ,  $(BAAB, i = j', j = i')$ ,  $(BABA, i = i', j = j')$ .  $E(\mathcal{D}_{ij}) = E(\mathcal{D}_{i'j'}) = \mu_{\text{between}}$ .  $\Sigma_{ij,i'j'} = \sigma_3^2$ . Its size is

$$m_4 = 4n_A n_B. \quad (\text{S.8})$$

**Case 5:**  $(ABAB, i = i', j \neq j' \text{ or } i \neq i', j = j')$ ,  $(ABBA, i = j', j \neq i' \text{ or } i \neq j', j = i')$ ,  $(BAAB, i = j', j \neq i' \text{ or } i \neq j', j = i')$ ,  $(BABA, i = i', j \neq j' \text{ or } i \neq i', j = j')$ .  $E(\mathcal{D}_{ij}) = E(\mathcal{D}_{i'j'}) = \mu_{\text{between}}$ .  $\Sigma_{ij,i'j'} = \sigma_4^2$ . Its size is

$$\mathbf{m}_5 = 4n_A n_B (n - 2). \quad (\text{S.9})$$

If there is no group difference, we have  $\delta_\mu = 0$ , so that Cases 1, 4 can be combined into Case I ( $i = i', j = j'$ ,  $\sigma_3^2 = \sigma_1^2$ ); and Cases 2, 3, 5 (marked in bold face) can be combined into Case II ( $i = i', j \neq j' \text{ or } i \neq i', j = j'$ ,  $\sigma_4^2 = \sigma_2^2$ ). In either case, we know that  $E(\mathcal{D}_{ij}) = E(\mathcal{D}_{i'j'}) = \mu_{\text{within}}$ , and

$$\Sigma_{ij,i'j'} = \begin{cases} \sigma_1^2, & m_I = m_1 + m_4 = 2n(n - 1). \\ \sigma_2^2, & m_{II} = m_2 + m_3 + m_5 = 4n(n - 1)(n - 2). \end{cases} \quad (\text{S.10})$$

As we mentioned in Section 3.3 of the main text, for most practical applications, both  $n_A$  and  $n_B$  are large, and the true effect,  $\delta_\mu$ , is small. Besides, we know that  $\sigma_3^2 - \sigma_1^2 = 0$  and  $\delta_{\sigma^2} := \sigma_4^2 - \sigma_2^2 = 0$  when  $\delta_\mu = 0$  (no group difference), therefore it is reasonable to assume that  $\delta_\mu$  decreases as a function of  $n$  and  $\delta_{\sigma^2} \rightarrow 0$  when  $n \rightarrow \infty$ . These conditions are summarized by Equation (3.15) in the main text, which is also copied below for convenience

$$\begin{aligned} n_A/n \rightarrow \lambda, \quad \lim_{n \rightarrow \infty} \sqrt{n} \delta_\mu(n) = c_\mu, \quad \lim_{n \rightarrow \infty} \sqrt{n} \delta_{\sigma^2}(n) = c_{\sigma^2}. \\ \lim_{n \rightarrow \infty} (\sigma_3^2(n) - \sigma_1^2(n)) = 0. \end{aligned} \quad (\text{S.11})$$

### S1.3 Large Sample Approximations of the Covariance Matrix of $\mathcal{D}$

Under the assumptions listed in Section S1.1 and Equation (S.11) (which is Equation (3.15) in the main text), we see that both Cases 1 and 4 are negligible compared with Cases 2, 3, and 5 (these three cases were marked in **bold face** in the previous list), because  $m_1, m_4 = O(n^2)$  and  $m_2, m_3, m_5 = O(n^3)$ . Asymptotically, the major component of covariance can be consolidated into the following three cases:

**Case 2:**  $AAAA$  or  $BBBB$ ;  $(i = i', j \neq j')$ ,  $(i = j', i' \neq j)$ ,  $(i \neq j', j = i')$ , or  $(i \neq i', j = j')$ .  $E(\mathcal{D}_{ij}) = E(\mathcal{D}_{i'j'}) = \mu_{\text{within}}$ .  $\Sigma_{ij,i'j'} = \sigma_2^2$ . Total number of cases:  $m_2 \approx 4n_A^3 + 4n_B^3$ .

**Case 3:**  $(AAAB, i = i' \text{ or } j = i')$ ,  $(AABA, i = j' \text{ or } j = j')$ ,  $(ABAA, i = i' \text{ or } i = j')$ ,  $(BAAA, j = i' \text{ or } j = j')$ .  $(E(\mathcal{D}_{ij}) = \mu_{\text{within}}, E(\mathcal{D}_{i'j'}) = \mu_{\text{between}})$  or  $(E(\mathcal{D}_{ij}) = \mu_{\text{between}}, E(\mathcal{D}_{i'j'}) = \mu_{\text{within}})$ .  $\Sigma_{ij,i'j'} = \sigma_2^2$ . Total number of cases:  $m_3 \approx 8nn_A n_B$ .

**Case 5:**  $(ABAB, i = i', j \neq j' \text{ or } i \neq i', j = j')$ ,  $(ABBA, i = j', j \neq i' \text{ or } i \neq j', j = i')$ ,  $(BAAB, i = j', j \neq i' \text{ or } i \neq j', j = i')$ ,  $(BABA, i = i', j \neq j' \text{ or } i \neq i', j = j')$ .  $E(\mathcal{D}_{ij}) = E(\mathcal{D}_{i'j'}) = \mu_{\text{between}}$ .  $\Sigma_{ij,i'j'} = \sigma_4^2$ . Total number of cases:  $m_5 = 4nn_A n_B$ .

As a special case, when there is no group difference, we only need to consider Case II, in which  $E(\mathcal{D}_{ij}) = E(\mathcal{D}_{i'j'}) = \mu_{\text{within}}$  and  $\Sigma_{ij,i'j'} = \sigma_2^2$ . The size of Case II is  $m_{II} = 4n(n-1)(n-2) \approx 4n^3$ .

### S1.4 Mean and Variance of Total Distance

Let  $H_n := 1'_n \mathcal{D}_n 1_n = \sum_{i=1}^n \sum_{j=1}^n \mathcal{D}_{n,ij}$  be the total squared distance. We will derive the mean and variance of  $H_n$  in this section.

According to Equation (S.4), we have

$$\begin{aligned} E(H_n) &= \mu_{\text{within}} 1'_n (J_n - I_n) 1_n + \delta_\mu 1'_n (1_A 1'_B + 1_B 1'_A) 1_n \\ &= \mu_{\text{within}} (n^2 - n) + 2\delta_\mu n_A n_B. \end{aligned} \quad (\text{S.12})$$

According to the classification of elements in  $\Sigma$  provided in Section S1.1, and  $\delta_{\sigma^2} := \sigma_4^2 - \sigma_2^2 = O(n^{-1/2})$ , as we assumed in Equation (3.15), we have

$$\begin{aligned} \text{var}(H_n) &= m_1 \sigma_1^2 + (m_2 + m_3) \sigma_2^2 + m_4 \sigma_3^2 + m_5 \sigma_4^2 \\ &= (2(n_A^2 + n_B^2) - 2n) \sigma_1^2 + 4(n_A^3 + n_B^3 - 3(n_A^2 + n_B^2) + 2n + 2n_A n_B (n-2)) \sigma_2^2 \\ &\quad + 4n_A n_B \sigma_3^2 + 4n_A n_B (n-2) \sigma_4^2 \\ &= \underbrace{4n^3 \sigma_2^2}_{O(n^3)} + \underbrace{4nn_A n_B \delta_{\sigma^2}}_{O(n^{2.5})} + \underbrace{2(n_A^2 + n_B^2) \sigma_1^2 - 12n^2 \sigma_2^2 + 4n_A n_B \sigma_3^2}_{O(n^2)} - \underbrace{8n_A n_B \delta_{\sigma^2}}_{O(n^{1.5})} - \underbrace{2n \sigma_1^2 + 8n \sigma_2^2}_{O(n)}. \end{aligned} \quad (\text{S.13})$$

Let  $H_{n,A} := 1'_A \mathcal{D}_n 1_A$  and  $H_{n,B} := 1'_B \mathcal{D}_n 1_B$  be the total squared distance within groups  $A$  and  $B$ , respectively. It is easy to see that

$$\begin{aligned} E(H_{n,A}) &= \mu_{\text{within}} (n_A^2 - n_A), \quad E(H_{n,B}) = \mu_{\text{within}} (n_B^2 - n_B). \\ \text{var}(H_{n,A}) &= 2n_A (n_A - 1) \sigma_1^2 + 4n_A (n_A - 1) (n_A - 2) \sigma_2^2 \\ &= 2n_A^2 \sigma_1^2 + 4(n_A^3 - 3n_A^2) \sigma_2^2 + O(n). \\ \text{var}(H_{n,B}) &= 2n_B (n_B - 1) \sigma_1^2 + 4n_B (n_B - 1) (n_B - 2) \sigma_2^2 \\ &= 2n_B^2 \sigma_1^2 + 4(n_B^3 - 3n_B^2) \sigma_2^2 + O(n). \end{aligned} \quad (\text{S.14})$$

Let  $H_{n,AB} := 2 \cdot 1'_A \mathcal{D}_n 1_B = H_n - H_{n,A} - H_{n,B}$  be the sum of off-diagonal squared distance. We can show that

$$\begin{aligned} E(H_{n,AB}) &= E(H_n) - E(H_{n,A}) - E(H_{n,B}) \\ &= 2\delta_\mu n_A n_B + \mu_{\text{within}}(n^2 - n) - \mu_{\text{within}}(n_A^2 - n_A + n_B^2 - n_B) \\ &= 2(\delta_\mu + \mu_{\text{within}})n_A n_B. \end{aligned} \quad (\text{S.15})$$

$$\begin{aligned} \text{var}(H_{n,AB}) &= m_4 \sigma_3^2 + m_5 \sigma_4^2 \\ &= 4n_A n_B \sigma_3^2 + 4n_A n_B (n-2) \sigma_4^2 = 4n_A n_B n \sigma_4^2 + O(n^2). \end{aligned} \quad (\text{S.16})$$

$$\begin{aligned} \text{cov}(H_{n,AB}, H_{n,A}) &= \frac{8n_A(n_A-1)n_B \sigma_2^2}{2} \\ &= 4n_A(n_A-1)n_B \sigma_2^2 = 4n_A^2 n_B \sigma_2^2 + O(n^2). \\ \text{cov}(H_{n,AB}, H_{n,B}) &= 4n_B(n_B-1)n_A \sigma_2^2 = 4n_A n_B^2 \sigma_2^2 + O(n^2). \end{aligned} \quad (\text{S.17})$$

$$\text{cov}(H_{n,AB}, H_{n,A} + H_{n,B}) = \frac{m_3 \sigma_2^2}{2} = 4n_A n_B (n-2) \sigma_2^2 = 4n_A n_B n \sigma_2^2 + O(n^2).$$

## S1.5 Asymptotic Mean and Variance of $F(\mathcal{D})$

Using the notations  $H_n$ ,  $H_{n,A}$ , and  $H_{n,B}$  defined in the previous section, we can re-write the proposed summary statistic,  $F(\mathcal{D}_n)$ , as follows

$$\begin{aligned} F(\mathcal{D}_n) &= (n-2) \frac{\text{Top}_n}{\text{Bottom}_n}. \\ \text{Bottom}_n &:= \frac{H_{n,A}}{n_A} + \frac{H_{n,B}}{n_B}, \quad \text{Top}_n := \frac{H_n}{n} - \frac{H_{n,A}}{n_A} - \frac{H_{n,B}}{n_B} = \frac{H_n}{n} - \text{Bottom}_n. \end{aligned} \quad (\text{S.18})$$

Below we provide Lemma S1 and Theorem S2, which describe some universal large sample properties of  $F(\mathcal{D})$  that are applicable to all distributional assumptions of the networks and the distance function.

**Lemma S1.** *Based on the assumptions listed earlier, we have*

$$\begin{aligned} E(\text{Bottom}_n) &= \mu_{\text{within}}(n-2), \quad E(\text{Top}_n) \approx 2c(\lambda - \lambda^2) \cdot \sqrt{n} + \mu_{\text{within}}. \\ \text{var}(\text{Bottom}_n) &= 4(n-6)\sigma_2^2 + 4\sigma_1^2 + O(n^{-1}). \\ \text{var}(\text{Top}_n) &= \begin{cases} 2\sigma_1^2 - 4\sigma_2^2 + O(n^{-1}), & \text{under } H_0. \\ 4\lambda(1-\lambda)c_{\sigma^2}\sqrt{n} + O(1), & \text{under } H_1. \end{cases} \\ \text{cov}(\text{Top}_n, \text{Bottom}_n) &= 8\sigma_2^2 - 2\sigma_1^2 + O(n^{-1}). \end{aligned} \quad (\text{S.19})$$

*In particular, the correlation between  $\text{Top}_n$  and  $\text{Bottom}_n$  converges to zero when  $n \rightarrow \infty$  under both  $H_0$  and  $H_1$ .*

*Proof.* Based on the assumptions listed in Equation (3.15), we know that  $\delta_\mu(n) \approx c_\mu \cdot n^{-1/2}$  and  $n_A/n \rightarrow \lambda \in (0, 1)$  for some constants  $c$  and  $\lambda$ . Based on Equations (S.12) and (S.14), we know that

$$\begin{aligned} \frac{E(H_n)}{n} &= 2\delta_\mu \cdot \frac{n_A n_B}{n} + \mu_{\text{within}}(n-1) \approx 2c(\lambda - \lambda^2) \cdot \sqrt{n} + \mu_{\text{within}}(n-1). \\ \frac{E(H_{n,A})}{n_A} &= \mu_{\text{within}}(n_A-1), \quad \frac{E(H_{n,B})}{n_B} = \mu_{\text{within}}(n_B-1). \end{aligned}$$

Therefore  $E(\text{Bottom}_n) = \mu_{\text{within}}(n-2)$ , and

$$\begin{aligned} E(\text{Top}_n) &= 2\delta_\mu \cdot \frac{n_A n_B}{n} + \mu_{\text{within}} \approx 2c(\lambda - \lambda^2) \cdot \sqrt{n} + \mu_{\text{within}}. \\ \text{var}(\text{Bottom}_n) &= 4(n-6)\sigma_2^2 + 4\sigma_1^2 + O(n^{-1}). \end{aligned}$$

It is easy to show that

$$\begin{aligned} \text{var}(\text{Bottom}_n) &= \frac{\text{var}(H_{n,A})}{n_A^2} + \frac{\text{var}(H_{n,B})}{n_B^2} \\ &= 4(n-6)\sigma_2^2 + 4\sigma_1^2 + O(n^{-1}). \end{aligned} \tag{S.20}$$

By definition

$$\begin{aligned} \text{Top}_n &= \frac{H_n}{n} - \frac{H_{n,A}}{n_A} - \frac{H_{n,B}}{n_B} = \left(\frac{1}{n} - \frac{1}{n_A}\right) H_{n,A} + \left(\frac{1}{n} - \frac{1}{n_B}\right) H_{n,B} + \frac{H_{n,AB}}{n} \\ &= -\frac{n_B}{nn_A} H_{n,A} - \frac{n_A}{nn_B} H_{n,B} + \frac{H_{n,AB}}{n}. \end{aligned} \tag{S.21}$$

Therefore

$$\begin{aligned} \text{var}(\text{Top}_n) &= \frac{n_B^2}{n^2 n_A^2} \text{var}(H_{n,A}) + \frac{n_A^2}{n^2 n_B^2} \text{var}(H_{n,B}) + \frac{\text{var}(H_{n,AB})}{n^2} \\ &\quad - \frac{2n_B}{n^2 n_A} \text{cov}(H_{n,AB}, H_{n,A}) - \frac{2n_A}{n^2 n_B} \text{cov}(H_{n,AB}, H_{n,B}) \\ &= \frac{n_B^2 (2n_A^2 \sigma_1^2 + 4(n_A^3 - 3n_A^2) \sigma_2^2 + O(n))}{n^2 n_A^2} \\ &\quad + \frac{n_A^2 (2n_B^2 \sigma_1^2 + 4(n_B^3 - 3n_B^2) \sigma_2^2 + O(n))}{n^2 n_B^2} \\ &\quad + \frac{4n_A n_B \sigma_3^2 + 4n_A n_B (n-2) \sigma_4^2}{n^2} \\ &\quad - \frac{2n_B (4n_A (n_A - 1) n_B \sigma_2^2)}{n^2 n_A} - \frac{2n_A (4n_B (n_B - 1) n_A \sigma_2^2)}{n^2 n_B} \\ &= \frac{4n_A n_B n (\sigma_2^2 + \sigma_4^2) + (n_A^2 + n_B^2) (2\sigma_1^2 - 12\sigma_2^2) + 4n_A n_B (\sigma_3^2 - 2\sigma_4^2)}{n^2} \\ &\quad - \frac{8(n_A n_B n - (n_A^2 + n_B^2)) \sigma_2^2}{n^2} + O(n^{-1}) \\ &= \frac{4n_A n_B n (\sigma_4^2 - \sigma_2^2) + (n_A^2 + n_B^2) (2\sigma_1^2 - 4\sigma_2^2) + 4n_A n_B (\sigma_3^2 - 2\sigma_4^2)}{n^2} + O(n^{-1}) \\ &= 4\lambda(1-\lambda)c_{\sigma^2}\sqrt{n} + (\lambda^2 + (1-\lambda)^2)(2\sigma_1^2 - 4\sigma_2^2) + 4\lambda(1-\lambda)(\sigma_3^2 - 2\sigma_4^2) + O(n^{-1}). \end{aligned} \tag{S.22}$$

$$\begin{aligned} \text{cov}(\text{Top}_n, \text{Bottom}_n) &= \text{cov}\left(-\frac{n_B}{nn_A} H_{n,A} - \frac{n_A}{nn_B} H_{n,B} + \frac{H_{n,AB}}{n}, \frac{H_{n,A}}{n_A} + \frac{H_{n,B}}{n_B}\right) \\ &= -\frac{n_B}{nn_A^2} \text{var}(H_{n,A}) - \frac{n_A}{nn_B^2} \text{var}(H_{n,B}) + \frac{\text{cov}(H_{n,AB}, H_{n,A})}{nn_A} + \frac{\text{cov}(H_{n,AB}, H_{n,B})}{nn_B} \\ &= -\frac{2n\sigma_1^2 + (8n_A n_B - 12n)\sigma_2^2}{n} + \frac{4((n_A - 1)n_B + (n_B - 1)n_A)\sigma_2^2}{n} + O(n^{-1}) \\ &= 8\sigma_2^2 - 2\sigma_1^2 + O(n^{-1}). \end{aligned} \tag{S.23}$$

Based on Equations (S.22), (S.23), and (S.20), we see that

$$\begin{aligned}\text{cor}(\text{Top}_n, \text{Bottom}_n) &= \frac{\text{cov}(\text{Top}_n, \text{Bottom}_n)}{\sqrt{\text{var}(\text{Top}_n)\text{var}(\text{Bottom}_n)}} \\ &= \frac{8\sigma_2^2 - 2\sigma_1^2 + O(n^{-1})}{\sqrt{O(n)}} = O(n^{-1/2}) \rightarrow 0.\end{aligned}\tag{S.24}$$

□

**Theorem S2.** *Based on the assumptions listed earlier, the asymptotic distribution of  $F(\mathcal{D})$  and  $\frac{\text{Top}_n}{\mu_{\text{within}}}$  are equivalent. More specifically, we assume that there exist a non-degenerate limiting distribution  $G_F(\cdot)$  and two sequences of real numbers  $a_n$  and  $b_n$  such that*

$$\frac{\text{Top}_n(\mathcal{D}_n) - a_n}{b_n} \xrightarrow{d} G_{\text{Top}_n}(\cdot),\tag{S.25}$$

under the assumptions stated in Section S1.3 and Equation (3.15).

We conclude that

$$\frac{F(\mathcal{D}_n)\mu_{\text{within}} - a_n}{b_n} \xrightarrow{d} G_{\text{Top}_n}(\cdot).$$

*Proof.* Let  $X_n := \frac{\text{Top}_n(\mathcal{D}_n) - a_n}{b_n}$ ,  $Y_n := \frac{(n-2)\mu_{\text{within}}}{\text{Bottom}(\mathcal{D}_n)}$ , and  $Z_n := \frac{F(\mathcal{D}_n)\mu_{\text{within}} - a_n}{b_n}$ . Apparently, we have

$$Z_n = X_n Y_n + \frac{a_n}{b_n} (Y_n - 1).$$

Based on Equation (S.19), we know that

$$E\left(\frac{1}{Y_n}\right) = 1, \quad \text{var}\left(\frac{1}{Y_n}\right) = O(n^{-1}),$$

which implies that  $\frac{1}{Y_n} \rightarrow 1$  in  $L^2$  and in probability. Using continuous mapping theorem, we know that  $Y_n \xrightarrow{p} 1$ , and  $\text{var}(Y_n) = O(n^{-1})$ .

Again based on Equation (S.19), we see that by letting

$$\begin{cases} a_n = \mu_{\text{within}}, & b_n = \sqrt{2\sigma_1^2 - 4\sigma_2^2} & (\text{under } H_0) \\ a_n = 2c_\mu\lambda(1-\lambda) \cdot \sqrt{n}, & b_n = 2\sqrt{\lambda(1-\lambda)c_{\sigma^2}n^{1/4}}, & (\text{under } H_1) \end{cases}$$

$X_n$  will be standardized asymptotically, namely,  $\lim_{n \rightarrow \infty} EX_n = 0$ ,  $\lim_{n \rightarrow \infty} \text{var}(X_n) = 1$ . Based on the assumption that  $G_F(\cdot)$  is non-degenerate, we know that other choices of  $a_n$  and  $b_n$  must be of the same order, namely, every such choice must satisfy

$$\begin{cases} a_n, b_n = O(1), & (\text{under } H_0) \\ a_n = O(n^{1/2}), & b_n = O(n^{1/4}), & (\text{under } H_1) \end{cases}$$

The above analysis implies that  $\frac{a_n}{b_n}$  is either of order  $O(1)$  (under  $H_0$ ) or  $O(n^{1/4})$  (under  $H_1$ ). Therefore

$$\text{var}\left(\frac{a_n}{b_n} (Y_n - 1)\right) = \frac{a_n^2}{b_n^2} \cdot \text{var}(Y_n) = \begin{cases} O(n^{-1}), & (\text{under } H_0) \\ O(n^{-1/2}), & (\text{under } H_1) \end{cases}\tag{S.26}$$

In either case, we see that  $\text{var}\left(\frac{a_n}{b_n}(Y_n - 1)\right) \rightarrow 0$  therefore  $\frac{a_n}{b_n}(Y_n - 1) \rightarrow 0$  in  $L^2$  and in probability. Using Slutsky's theorem, we conclude that

$$\frac{F(\mathcal{D}_n)\mu_{\text{within}} - a_n}{b_n} := Z_n = X_n Y_n + \frac{a_n}{b_n}(Y_n - 1) \xrightarrow{d} G_F(\cdot).$$

□

Based on Lemma S1 and Theorem S2, we conclude that

$$\begin{aligned} E(F(\mathcal{D}_n)) &= \begin{cases} 1, & (\text{under } H_0) \\ 1 + \frac{2c\lambda(1-\lambda)\sqrt{n}}{\mu_{\text{within}}} + o(n^{1/2}), & (\text{under } H_1) \end{cases}, \\ \text{var}(F(\mathcal{D}_n)) &= \begin{cases} \frac{2\sigma_1^2 - 4\sigma_2^2}{\mu_{\text{within}}^2}, & \text{under } H_0, \\ \frac{4\lambda(1-\lambda)c_{\sigma^2}\sqrt{n}}{\mu_{\text{within}}^2} + o(n^{1/2}), & \text{under } H_1. \end{cases} \end{aligned} \quad (\text{S.27})$$

Which finishes the proof of the first half of Theorem 2 in the main text.

## S1.6 Expectation and Variance of the Permuted $F(\mathcal{D})$

To prove the second half of Theorem 2 in the main text, we need to compute the expectation and variance of  $F(\pi(\mathcal{D}_n))$ , which is the  $F$ -statistic computed after applying a permutation  $\pi$  to the  $n$  samples.

To this end, we need the following terminologies and assumptions.

1. In this section, we assume that  $\pi$  is a random permutation uniformly sampled from  $\text{sym}(n)$ , the collection of all permutations of  $n$  labels.
2. For convenience, let us define  $\kappa(\pi) : \text{sym}(n) \rightarrow \{0, 1, \dots, n_A\}$  to be the number of samples in group  $A$  that remains in group  $A$  after the permutation. Due to the uniformity assumption, it is easy to see that  $\kappa(\pi)$  follows a hypergeometric distribution  $\text{HypGeo}(n, n_A, n_A)$ , such that (for  $n \geq 4$ )

$$\begin{aligned}
P(\kappa(\pi) = k) &= \frac{\binom{n_A}{k} \binom{n_B}{n_A-k}}{\binom{n}{n_A}}, & E(\kappa(\pi)) &= \frac{n_A}{n}, \\
E(\kappa(\pi)^2) &= \text{var}(\kappa(\pi)^2) + (E(\kappa(\pi)))^2 = \frac{n_A^2(n - n_A)(n - n_A)}{n^2(n - 1)} + \frac{n_A^4}{n^2} \\
&= \frac{n_A^4}{n^2} + \frac{n_A^2 n_B^2}{n^3} + O(1). \\
E(\kappa(\pi)^3) &= \frac{n_A^2}{n} + \frac{3n_A^2(n_A - 1)^2}{n(n - 1)} + \frac{n_A^2(n_A - 1)^2(n_A - 2)^2}{n(n - 1)(n - 2)} \\
&= \frac{n_A^2(n_A^4 - 6n_A^3 + 3n_A^2n + 7n_A^2 - 6nn_A + n^2)}{n(n - 1)(n - 2)} \\
&= \frac{n_A^6}{n^3} + \frac{3n_A^4 n_B^2}{n^4} + O(n). \\
E(\kappa(\pi)^4) &= \frac{n_A^2}{n} + \frac{7n_A^2(n_A - 1)^2}{n(n - 1)} + \frac{6n_A^2(n_A - 1)^2(n_A - 2)^2}{n(n - 1)(n - 2)} \\
&\quad + \frac{n_A^2(n_A - 1)^2(n_A - 2)^2(n_A - 3)^2}{n(n - 1)(n - 2)(n - 3)} \\
&= \frac{n_A^2((n_A - 1)^2(n_A - 2)^2(n_A - 3)^2 + 6(n_A - 1)^2(n_A - 2)^2(n - 3) + O(n^4))}{n^4 - 6n^3 + O(n^2)} \\
&= \frac{n_A^8 - 12n_A^7 + 6nn_A^6 + O(n^6)}{n^4 - 6n^3 + O(n^2)} = \frac{n_A^8}{n^4} + \frac{6n_A^6 n_B^2}{n^5} + O(n^3).
\end{aligned} \tag{S.28}$$

By definition, we know that there are  $\kappa(\pi)$  samples from group  $A$  and  $n_A - \kappa(\pi)$  samples from group  $B$  in the first  $n_A$  samples after  $\pi$ -permutation. The top-left  $(n_A \times n_A)$ -dimensional submatrix of  $\mathcal{D}_n$  contains  $n_A$  zeros (diagonal elements),  $\kappa(\pi)^2 + (n_A - \kappa(\pi))^2 - n_A$  within-group distances, and  $n_A^2 - \kappa(\pi)^2 - (n_A - \kappa(\pi))^2 = 2\kappa(\pi)(n_A - \kappa(\pi))$  between-group distances.

Similarly, there are  $n_A - \kappa(\pi)$  samples from group  $A$  and  $n_B - n_A + \kappa(\pi)$  samples from group  $B$  in the rest  $n_B$  samples after  $\pi$ -permutation. The bottom-right  $(n_B \times n_B)$ -dimensional submatrix of  $\mathcal{D}_n$  contains  $n_B$  zeros,  $(n_A - \kappa(\pi))^2 + (n_B - n_A + \kappa(\pi))^2 - n_B$  within-group distances, and  $n_B^2 - (n_A - \kappa(\pi))^2 - (n_B - n_A + \kappa(\pi))^2 = 2(n_A - \kappa(\pi))(n_B - n_A + \kappa(\pi))$  between-group distances. Using Equation (S.12), we know

$$\begin{aligned}
\frac{E(H_{n,A}(\pi(\mathcal{D}_n)) | \kappa(\pi) = k)}{n_A} &= -2\delta_\mu \left( \frac{k^2}{n_A} - k \right) + \mu_{\text{within}}(n_A - 1), \\
\frac{E(H_{n,B}(\pi(\mathcal{D}_n)) | \kappa(\pi) = k)}{n_B} &= -2\delta_\mu (n_A - k)^2 + 2\delta_\mu n_B (n_A - k) + \mu_{\text{within}}(n_B - 1) \\
&= -2\delta_\mu \left( \frac{k^2}{n_B} + \left(1 - \frac{2n_A}{n_B}\right)k + \frac{n_A^2}{n_B} - n_A \right) + \mu_{\text{within}}(n_B - 1). \\
E(\text{Bottom}_n(\pi(\mathcal{D}_n)) | \kappa(\pi) = k) &= E \left( \frac{H_{n,A}}{n_A} + \frac{H_{n,B}}{n_B} \middle| \kappa(\pi) = k \right) \\
&= \mu_{\text{within}}(n - 2) - 2\delta_\mu \left( k^2 \left( \frac{1}{n_A} + \frac{1}{n_B} \right) - \frac{2n_A k}{n_B} + \frac{n_A^2 - n_A n_B}{n_B} \right) \\
&= \mu_{\text{within}}(n - 2) - 2\delta_\mu \cdot \frac{nk^2 - 2n_A^2 k + n_A^3 - n_A^2 n_B}{n_A n_B}.
\end{aligned} \tag{S.29}$$

On the other hand, we know that permutation does not change the sum of total squared distance, namely,

$H(\pi(\mathcal{D}_n)) = H(\mathcal{D}_n)$  for all  $\pi \in \text{sym}(n)$ . Therefore, we have

$$\begin{aligned}
E(\text{Top}_n(\pi(\mathcal{D}_n)) | \kappa(\pi) = k) &= \frac{E(H_n)}{n} - E(\text{Bottom}_n(\pi(\mathcal{D}_n)) | \kappa(\pi) = k) \\
&= \mu_{\text{within}} + 2\delta_\mu \left( \frac{n_A n_B}{n} + \frac{nk^2 - 2n_A^2 k + n_A^3 - n_A^2 n_B}{n_A n_B} \right) \\
&= \mu_{\text{within}} + 2\delta_\mu \left( \frac{n^2 k^2 - 2n n_A^2 k + n_A^4}{n n_A n_B} \right) \\
&\approx \mu_{\text{within}} + 2c_\mu \sqrt{n} \left( \frac{1}{\lambda(1-\lambda)} \cdot \frac{k^2}{n^2} - \frac{2\lambda}{1-\lambda} \frac{k}{n} + \frac{\lambda^3}{1-\lambda} \right).
\end{aligned} \tag{S.30}$$

Using Equation (S.28), the unconditional expectation of  $\text{Top}_n(\pi(\mathcal{D}_n))$  is

$$\begin{aligned}
E(\text{Top}_n(\pi(\mathcal{D}_n))) &= E_k(E(\text{Top}_n(\pi(\mathcal{D}_n)) | \kappa(\pi) = k)) \\
&\approx \mu_{\text{within}} + 2c_\mu \sqrt{n} \left( \frac{1}{\lambda(1-\lambda)} \cdot \frac{E(k^2)}{n^2} - \frac{2\lambda}{1-\lambda} \frac{E(k)}{n} + \frac{\lambda^3}{1-\lambda} \right) \\
&= \mu_{\text{within}} + 2c_\mu \sqrt{n} \left( \frac{1}{\lambda(1-\lambda)} \cdot \lambda^4 - \frac{2\lambda}{1-\lambda} \lambda^2 + \frac{\lambda^3}{1-\lambda} \right) \\
&= \mu_{\text{within}}.
\end{aligned} \tag{S.31}$$

Let us use  $\langle X, Y \rangle_k$  as a shortcut for the covariance between two random variables  $X$  and  $Y$  conditionally on  $\kappa(\pi) = k$ . For example

$$\langle H_{n,A}, H_{n,A} \rangle := \text{var}(H_{n,A}(\pi(\mathcal{D}_n)) | \kappa(\pi) = k), \quad \langle H_n, \text{Bottom}_n \rangle_k := \text{cov}(H_n, \text{Bottom}_n(\pi(\mathcal{D}_n)) | \kappa(\pi) = k).$$

Notice that after permutation, the first  $n_A$  samples contain  $k$  samples in group  $A$  and  $n_A - k$  samples from group  $B$ , using Equation (S.13), we obtain

$$\begin{aligned}
\langle H_{n,A}, H_{n,A} \rangle &= \underbrace{4n_A^3 \sigma_2^2}_{O(n^3)} + \underbrace{4n_A(-k^2 + n_A k) \delta_{\sigma^2}}_{O(n^{2.5})} \\
&\quad + \underbrace{(4k^2 - 4n_A k + 2n_A^2) \sigma_1^2 - 12n_A^2 \sigma_2^2 + (-4k^2 + 4n_A k) \sigma_3^2}_{O(n^2)} + O(n^{1.5}).
\end{aligned} \tag{S.32}$$

Similarly, we can derive

$$\begin{aligned}
\langle H_{n,B}, H_{n,B} \rangle &= 4n_B^3 \sigma_2^2 + 4n_B(-k^2 + (2n_A - n_B)k + n_A n_B - n_A^2) \delta_{\sigma^2} \\
&\quad + (4k^2 + 4(n_B - 2n_A)k + 4n_A^2 + 2n_B^2 - 4n_A n_B) \sigma_1^2 - 12n_B^2 \sigma_2^2 \\
&\quad + 4(-k^2 + (2n_A - n_B)k + n_A n_B - n_A^2) \sigma_3^2 + O(n^{1.5}).
\end{aligned} \tag{S.33}$$

Consequently

$$\begin{aligned}
\langle \text{Bottom}_n, \text{Bottom}_n \rangle_k &= \frac{\langle H_{n,A}, H_{n,A} \rangle}{n_A^2} + \frac{\langle H_{n,B}, H_{n,B} \rangle}{n_B^2} \\
&= 4n\sigma_2^2 + \frac{4(-nk^2 + 2n_A^2 k + n_A^2 n_B - n_A^3)}{n_A n_B} \cdot \delta_{\sigma^2} \\
&\quad + 4\sigma_1^2 \cdot \frac{(n_A^2 + n_B^2)k^2 + n_A(n_A n_B - 2n_A^2 - n_B^2)k + n_A^2(n_A^2 + n_B^2 - n_A n_B)}{n_A^2 n_B^2} - 24\sigma_2^2 \\
&\quad + 4\sigma_3^2 \cdot \frac{-(n_A^2 + n_B^2)k^2 + n_A(2n_A^2 + n_B^2 - n_A n_B)k + n_A^3(n_B - n_A)}{n_A^2 n_B^2} + O(n^{-1/2}).
\end{aligned} \tag{S.34}$$

Now we can derive the conditional mean and variance/covariance of  $H_{n,AB}(\pi(\mathcal{D}_n))$ . By the definition of  $\kappa$ ,  $H_{n,AB}(\pi(\mathcal{D}_n))$  is the summation of those two types of squared distances  $\mathcal{D}_{n,ij}$ :

1. Either  $i, j \in A$  or  $i, j \in B$ . The first case has  $2k(n_A - k)$  items, and the second case has  $2(n_A - k)(n_B - n_A + k)$  items, so there are  $\tilde{m}_1 := 2(n_A n_B - n_A^2 + (3n_A - n_B)k - 2k^2)$  items in total.  $E(\mathcal{D}_{n,ij} | \kappa(\pi) = k) = \mu_{\text{within}}$ ,  $\text{var}(\mathcal{D}_{n,ij} | \kappa(\pi) = k) = \sigma_1^2$ .
2. Either  $i \in A$  and  $j \in B$  or  $i \in B$ ,  $j \in A$ . There are  $\tilde{m}_2 := 2((n_A - k)^2 + k(n_B - n_A + k))$  items in total.  $E(\mathcal{D}_{n,ij} | \kappa(\pi) = k) = \mu_{\text{within}} + \delta_\mu$ ,  $\text{var}(\mathcal{D}_{n,ij} | \kappa(\pi) = k) = \sigma_3^2$ .

We see that

$$\begin{aligned}
E(H_{n,AB}(\pi(\mathcal{D}_n)) | \kappa(\pi) = k) &= \tilde{m}_1 \mu_{\text{within}} + \tilde{m}_2 (\mu_{\text{within}} + \delta_\mu) \\
&= 2(n_A n_B - n_A^2 + (3n_A - n_B)k - 2k^2) \mu_{\text{within}} \\
&\quad + 2(n_A^2 + (n_B - 3n_A)k + 2k^2) (\mu_{\text{within}} + \delta_\mu) \\
&= 2n_A n_B \mu_{\text{within}} + 2(n_A^2 + (n_B - 3n_A)k + 2k^2) \delta_\mu.
\end{aligned} \tag{S.35}$$

Because  $H_{n,AB}$  summarizes all the *off-diagonal* elements in  $\mathcal{D}_n$ , we know that  $i \neq j$ ,  $i' \neq j'$ , therefore the covariance between  $\mathcal{D}_{n,ij}$  and  $\mathcal{D}_{n,i'j'}$  can be classified into the following cases.

1. Both  $(i, j)$  and  $(i', j')$  are in Case (a).

$$\text{cov}(\mathcal{D}_{n,ij}, \mathcal{D}_{n,i'j'}) = \begin{cases} \sigma_1^2, & i = i', j = j' \text{ or } i = j', j = i'; \text{ a total of } 2\tilde{m}_1 \text{ cases.} \\ \sigma_2^2, & i = i', j \neq j' \text{ or } i = j', j \neq i'; \text{ a total of } \tilde{m}_{1b} \text{ cases.} \\ 0, & \text{otherwise.} \end{cases}$$

$$\begin{aligned}
\tilde{m}_{1b} &:= 4(k(n_A - k)(n_A - 2) + (n_A - k)(n_B - n_A + k)(n_B - 2)) \\
&= 4(n_A - k)(k(n - 4) + (n_B - n_A)(n_B - 2)).
\end{aligned}$$

2. Both  $(i, j)$  and  $(i', j')$  are in Case (b).

$$\text{cov}(\mathcal{D}_{n,ij}, \mathcal{D}_{n,i'j'}) = \begin{cases} \sigma_3^2, & i = i', j = j'. \text{ A total of } 2\tilde{m}_2 \text{ cases.} \\ \sigma_4^2, & i = i', j \neq j', \text{ or } i \neq i', j = j'. \text{ A total of } \tilde{m}_{2b} \text{ cases.} \\ 0, & \text{otherwise.} \end{cases}$$

$$\tilde{m}_{2b} := 8(n_A - k)^2(n_A - k - 1) + 4k(n_B - n_A + k)(n_B - n_A + 2k - 2)$$

3.  $(i, j)$  and  $(i', j')$  are of two different cases.

$$\text{cov}(\mathcal{D}_{n,ij}, \mathcal{D}_{n,i'j'}) = \begin{cases} \sigma_2^2, & \text{one of } (i, j) \text{ equals one of } (i', j'). \text{ A total of } \tilde{m}_3 \text{ cases.} \\ 0, & \text{otherwise.} \end{cases}$$

$$\begin{aligned}
\tilde{m}_3 &:= 4(k(n_A - k)n_B + (n_A - k)(n_B - n_A + k)n_A) \\
&= 8(n_A - k)(kn + n_A(n_B - n_A)) \\
&= 8(2n_A^2 k - nk^2 + n_A^2(n_B - n_A)).
\end{aligned}$$

Therefore, we have

$$\begin{aligned}
\text{var} \left( H_{n,AB}(\pi(\mathcal{D}_n)) \middle| \kappa(\pi) = k \right) &= 2\tilde{m}_1\sigma_1^2 + (\tilde{m}_{1b} + \tilde{m}_3)\sigma_2^2 + 2\tilde{m}_2\sigma_3^2 + \tilde{m}_{2b}\sigma_4^2 \\
&\approx (\tilde{m}_{1b} + \tilde{m}_3)\sigma_2^2 + \tilde{m}_{2b}\sigma_4^2 \\
&\approx (12n(n_A k - k^2) + 4(n_A - k)(n_B - n_A)(n + n_A))\sigma_2^2 \\
&\quad + \tilde{m}_{2b}\sigma_4^2.
\end{aligned} \tag{S.36}$$

The conditional covariance between  $H_{n,A}$  and  $H_{n,AB}$  can be derived in this way.  $\text{cov}(D_{ij}, D_{i'j'})$  used in this covariance can be classified as

1. Type  $A_1 A_1 A_1 A_2$  or  $B_1 B_1 B_1 B_2$ ,  $i = i'$ , plus the permuted versions of them. The total number of  $\text{cov}(D_{ij}, D_{i'j'})$  in this category is

$$\begin{aligned}
\tilde{m}_{4a} &:= 4(k(k-1)(n_A - k) + (n_A - k)(n_A - k - 1)(n_B - n_A + k)) \\
&= 4(n_A - k)(k(2n_A - n_B - 2) + n_A n_B - n_A^2 - n_B + n_A) \\
&= 4((n_B - 2n_A + 2)k^2 + (3n_A^2 - 2n_A n_B + n_B - 3n_A)k + n_A(n_A - 1)(n_B - n_A)) \\
&= (4n_B - 8n_A + 8)k^2 + (12n_A^2 - 8n_A n_B + 4n_B - 12n_A)k + 4n_A(n_A - 1)(n_B - n_A).
\end{aligned}$$

The covariance is  $\sigma_2^2$ .

2. Type  $A_1 B_1 A_1 A_2$  with  $i = i'$ ;  $A_1 B_1 B_1 B_2$  with  $j = i'$ ;  $A_1 A_1 A_1 B_2$  with either  $i = i'$  or  $j = i'$ ;  $B_1 B_1 A_2 B_1$ , with either  $i = i'$  or  $j = i'$ ; plus the permuted versions of them. The total number of  $\text{cov}(D_{ij}, D_{i'j'})$  in this category is

$$\begin{aligned}
\tilde{m}_{4b} &:= 4(k(n_A - k)^2 + k(n_A - k)(n_B - n_A + k) + k(k-1)(n_B - n_A + k) + (n_A - k)^2(n_A - k - 1)) \\
&= 4(n_A - 1)(2k^2 + (n_B - 3n_A)k + n_A^2) \\
&= (8n_A - 8)k^2 + 4(n_A - 1)(n_B - 3n_A)k + 4n_A^2(n_A - 1) \\
&= (8n_A - 8)k^2 + (-12n_A^2 + 4n_A n_B - 4n_B + 12n_A)k + 4n_A^2(n_A - 1).
\end{aligned}$$

The covariance is  $\sigma_2^2$ .

3. Type  $A_1 B_1 A_1 B_2$  with  $i = i'$ ;  $A_1 B_1 A_2 B_1$  with  $j = j'$ , plus the permuted versions of them. The total number of  $\text{cov}(D_{ij}, D_{i'j'})$  in this category is

$$\tilde{m}_{4c} := 4k(n_A - k)n_B.$$

The covariance is  $\sigma_4^2$ .

Based on the above classification, we see that

$$\begin{aligned}
\tilde{m}_{4ab} &:= \tilde{m}_{4a} + \tilde{m}_{4b} = 4n_B(k^2 - n_A k + n_A(n_A - 1)). \\
\langle H_{n,A}, H_{n,AB} \rangle_k &:= \text{cov}(H_{n,A}, H_{n,AB}(\pi(\mathcal{D}_n)) \middle| \kappa(\pi) = k) = \tilde{m}_{4ab}\sigma_2^2 + \tilde{m}_{4c}\sigma_4^2 \\
&= 4n_B((n_A^2 - n_A)\sigma_2^2 - (k^2 - n_A k)\delta_{\sigma^2}).
\end{aligned} \tag{S.37}$$

Due to the symmetry between set  $A$  and  $B$ , we can derive the conditional covariance between  $H_{n,B}$  and  $H_{n,AB}$  by swapping  $n_A$  and  $n_B$ , and replacing  $k$  with  $n_B - n_A + k$ .

$$\begin{aligned}
\tilde{m}_{5ab} &:= 4n_A \left( (n_B - n_A + k)^2 - n_B(n_B - n_A + k) + n_B(n_B - 1) \right) \\
&= 4n_A \left( k^2 + (n_B - 2n_A)k + n_A^2 + n_B^2 - n_A n_B - n_B \right). \\
\tilde{m}_{5c} &:= 4(n_B - n_A + k)(n_B - (n_B - n_A + k))n_A \\
&= 4n_A \left( -k^2 + (2n_A - n_B)k + n_A n_B - n_A^2 \right). \\
\langle H_{n,B}, H_{n,AB} \rangle_k &= \tilde{m}_{5ab} \sigma_2^2 + \tilde{m}_{5c} \sigma_4^2 \\
&= 4n_A \left( (n_B^2 - n_B) \sigma_2^2 - (k^2 + (n_B - 2n_A)k + n_A^2 - n_A n_B) \delta_{\sigma^2} \right).
\end{aligned} \tag{S.38}$$

Recall that  $H_n := H_{n,A} + H_{n,B} + H_{n,AB}$  and  $\text{Bottom}_n(\pi(\mathcal{D}_n)) = \frac{H_{n,A}(\pi(\mathcal{D}_n))}{n_A} + \frac{H_{n,B}(\pi(\mathcal{D}_n))}{n_B}$ , therefore

$$\begin{aligned}
\langle H_n, \text{Bottom}_n \rangle_k &= \frac{\langle H_{n,A}, H_{n,A} \rangle_k + 0 + \langle H_{n,AB}, H_{n,A} \rangle_k}{n_A} \\
&\quad + \frac{0 + \langle H_{n,B}, H_{n,B} \rangle_k + \langle H_{n,AB}, H_{n,B} \rangle_k}{n_B} \\
&= 4n_A^2 \sigma_2^2 + 4(-k^2 + n_A k) \delta_{\sigma^2} \\
&\quad + \left( \frac{4k^2}{n_A} - 4k + 2n_A \right) \sigma_1^2 - 12n_A \sigma_2^2 + \left( -\frac{4k^2}{n_A} + 4k \right) \sigma_3^2 \\
&\quad + 4n_B \left( (n_A - 1) \sigma_2^2 - \left( \frac{k^2}{n_A} - k \right) \delta_{\sigma^2} \right) \\
&\quad + 4n_B^2 \sigma_2^2 + 4(-k^2 + (2n_A - n_B)k + n_A n_B - n_A^2) \delta_{\sigma^2} \\
&\quad + \left( \frac{4k^2}{n_B} + 4\left(1 - \frac{2n_A}{n_B}\right)k + \frac{4n_A^2}{n_B} + 2n_B - 4n_A \right) \sigma_1^2 - 12n_B \sigma_2^2 \\
&\quad + 4 \left( -\frac{k^2}{n_B} + \left( \frac{2n_A}{n_B} - 1 \right) k + n_A - \frac{n_A^2}{n_B} \right) \sigma_3^2 + O(n^{1/2}) \\
&\quad + 4n_A \left( (n_B - 1) \sigma_2^2 - \left( \frac{k^2}{n_B} + \left( 1 - \frac{2n_A}{n_B} \right) k + \frac{n_A^2}{n_B} - n_A \right) \delta_{\sigma^2} \right) \\
&= 4 \left( (n^2 - 4n) \sigma_2^2 + \left( -\frac{n^2 k^2}{n_A n_B} + \frac{2n_A n k}{n_B} + \frac{n_A n_B^2 - n_A^3}{n_B} \right) \delta_{\sigma^2} \right) \\
&\quad + \left( \frac{4n k^2}{n_A n_B} - \frac{8n_A k}{n_B} + \frac{4n_A^2}{n_B} + 2n_B - 2n_A \right) \sigma_1^2 \\
&\quad + 4 \left( \frac{-n k^2}{n_A n_B} + \frac{2n_A k}{n_B} + n_A - \frac{n_A^2}{n_B} \right) \sigma_3^2.
\end{aligned} \tag{S.39}$$

Now we can derive the conditional variance of  $\text{Top}_n(\pi(\mathcal{D}_n))$ , which is denoted by

$$\langle \text{Top}_n, \text{Top}_n \rangle_k := \text{var} \left( \text{Top}_n(\pi(\mathcal{D}_n)) \middle| \kappa(\pi) = k \right).$$

Recall that  $\text{Top}_n := \frac{H_n}{n} - \frac{H_{n,A}}{n_A} - \frac{H_{n,B}}{n_B} = \frac{H_n}{n} - \text{Bottom}_n$ , therefore

$$\begin{aligned}
\langle \text{Top}_n, \text{Top}_n \rangle_k &= \frac{\text{var}(H_n)}{n^2} + \langle \text{Bottom}_n, \text{Bottom}_n \rangle_k - \frac{2}{n} \langle H_n, \text{Bottom}_n \rangle_k \\
&= 4n\sigma_2^2 + \frac{4n_A n_B}{n} \delta_{\sigma^2} + \frac{2(n_A^2 + n_B^2)}{n^2} \sigma_1^2 - 12\sigma_2^2 + \frac{4n_A n_B}{n^2} \sigma_3^2 \\
&\quad + 4n\sigma_2^2 + \frac{4(-nk^2 + 2n_A^2 k + n_A^2 n_B - n_A^3)}{n_A n_B} \cdot \delta_{\sigma^2} \\
&\quad + 4\sigma_1^2 \cdot \frac{(n_A^2 + n_B^2)k^2 + n_A(n_A n_B - 2n_A^2 - n_B^2)k + n_A^2(n_A^2 + n_B^2 - n_A n_B)}{n_A^2 n_B^2} - 24\sigma_2^2 \\
&\quad + 4\sigma_3^2 \cdot \frac{-(n_A^2 + n_B^2)k^2 + n_A(2n_A^2 + n_B^2 - n_A n_B)k + n_A^3(n_B - n_A)}{n_A^2 n_B^2} \\
&\quad - 8 \left( (n-4)\sigma_2^2 + \left( -\frac{nk^2}{n_A n_B} + \frac{2n_A k}{n_B} + \frac{n_A n_B^2 - n_A^3}{n n_B} \right) \delta_{\sigma^2} \right) \\
&\quad + \left( -\frac{8k^2}{n_A n_B} + \frac{16n_A k}{n n_B} - \frac{8n_A^2}{n n_B} - 4\frac{n_B}{n} + 4\frac{n_A}{n} \right) \sigma_1^2 \\
&\quad + 8 \left( \frac{k^2}{n_A n_B} - \frac{2n_A k}{n n_B} - \frac{n_A}{n} + \frac{n_A^2}{n n_B} \right) \sigma_3^2 + O(n^{-1/2}) \\
&= -4\sigma_2^2 + \frac{4(n^2 k^2 - 2n n_A^2 k + 2n_A^4 - n n_A^3 - n_A^2 n_B^2 + n n_A^2 n_B)}{n n_A n_B} \delta_{\sigma^2} \\
&\quad + \frac{1}{n^2 n_A^2 n_B^2} \left( 4n^2(n_A - n_B)^2 k^2 + 4n n_A(3n_A^2 n_B - 2n_A^3 - n_B^3)k \right. \\
&\quad \left. + n_A^2(4n_A^4 - 4n_A^3 n_B - 2n_A^2 n_B^2 + 4n_A n_B^3 + 2n_B^4) \right) \sigma_1^2 \\
&\quad + \frac{4}{n^2 n_A^2 n_B^2} \left( -n^2(n_A - n_B)^2 k^2 + n n_A(2n_A^3 - 3n_A^2 n_B + n_B^3)k \right. \\
&\quad \left. + n_A^4(-n_A^2 + n_B^2 + n_A n_B) \right) \sigma_3^2 + O(n^{-1/2}).
\end{aligned} \tag{S.40}$$

Based on Equation (S.28), we know that  $E(k) = \frac{n_A^2}{n}$  and  $E(k^2) = \frac{n_A^4}{n^2} + O(n)$ . Based on the Assumption (3.15), we know that  $\sigma_3^2(n) - \sigma_1^2(n) = o(1)$ . Therefore

$$\begin{aligned}
E\langle \text{Top}_n, \text{Top}_n \rangle_k &= -4\sigma_2^2 + \frac{4(n_A^4 - 2n_A^4 + 2n_A^4 - n n_A^3 - n_A^2 n_B^2 + n n_A^2 n_B)}{n n_A n_B} \delta_{\sigma^2} \\
&\quad + \frac{1}{n^2 n_A^2 n_B^2} \left( 4(n_A - n_B)^2 n_A^4 + 4n_A^3(3n_A^2 n_B - 2n_A^3 - n_B^3) \right. \\
&\quad \left. + n_A^2(4n_A^4 - 4n_A^3 n_B - 2n_A^2 n_B^2 + 4n_A n_B^3 + 2n_B^4) \right) \sigma_1^2 \\
&\quad + \frac{4}{n^2 n_A^2 n_B^2} \left( -(n_A - n_B)^2 n_A^4 + n_A^3(2n_A^3 - 3n_A^2 n_B + n_B^3) \right. \\
&\quad \left. + n_A^3(-n_A^3 - n_A^2 n_B + n_A n_B^2 + 2n_B^3) \right) \sigma_3^2 + O(n^{-1/2}) \\
&= -4\sigma_2^2 + \frac{2(n_A^2 + n_B^2)\sigma_1^2}{n^2} + \frac{4n_A n_B \sigma_3^2}{n^2} + O(n^{-1/2}) \\
&= 2\sigma_1^2 - 4\sigma_2^2 + \frac{4n_A n_B}{n^2} (\sigma_3^2 - \sigma_1^2) + O(n^{-1/2}) = 2\sigma_1^2 - 4\sigma_2^2 + o(1).
\end{aligned} \tag{S.41}$$

Based on Equations (S.30) and (S.28), we know that

$$\begin{aligned}
\frac{E(\kappa^4)}{n^4} - \frac{4\lambda^2 E(\kappa^3)}{n^3} + 4\lambda^4 \frac{E(\kappa^2)}{n^2} &= \frac{n_A^8}{n^8} + \frac{6n_A^6 n_B^2}{n^9} - 4\lambda^2 \left( \frac{n_A^6}{n^6} + \frac{3n_A^4 n_B^2}{n^7} \right) + 4\lambda^4 \left( \frac{n_A^4}{n^4} + \frac{n_A^2 n_B^2}{n^5} \right) + O(n^{-2}) \\
&= \lambda^8 - \frac{2\lambda^6(1-\lambda)^2}{n} + O(n^{-2}). \\
\frac{E(\kappa^2)}{n^2} - 2\lambda^2 \cdot \frac{E(\kappa)}{n} &= \frac{n_A^4}{n^4} + \frac{n_A^2 n_B^2}{n^5} - 2\lambda^2 \frac{n_A^2}{n^2} = -\lambda^4 + \frac{\lambda^2(1-\lambda)^2}{n} + O(n^{-2}). \\
\left( \frac{E(\kappa^2)}{n^2} - 2\lambda^2 \cdot \frac{E(\kappa)}{n} \right)^2 &= \lambda^8 - \frac{2\lambda^6(1-\lambda)^2}{n} + O(n^{-2}). \\
\text{var} \left( \frac{\kappa^2}{n^2} - 2\lambda^2 \cdot \frac{\kappa}{n} \right) &= E \left( \frac{\kappa^4}{n^4} - 4\lambda^2 \cdot \frac{\kappa^3}{n^3} + 4\lambda^4 \cdot \frac{\kappa^2}{n^2} \right) - \left( \frac{E(\kappa^2)}{n^2} - 2\lambda^2 \cdot \frac{E(\kappa)}{n} \right)^2 \\
&= \lambda^8 - \frac{2\lambda^6(1-\lambda)^2}{n} - \left( \lambda^8 - \frac{2\lambda^6(1-\lambda)^2}{n} \right) + O(n^{-2}) \\
&= O(n^{-2}).
\end{aligned} \tag{S.42}$$

Hence

$$\begin{aligned}
\text{var} \left( E \left( \text{Top}_n(\pi(\mathcal{D}_n)) \middle| \kappa(\pi) = k \right) \right) &= \frac{4c_\mu^2 n}{\lambda^2(1-\lambda)^2} \text{var} \left( \frac{\kappa^2}{n^2} - 2\lambda^2 \cdot \frac{\kappa}{n} \right) \\
&= O(n^{-1}).
\end{aligned} \tag{S.43}$$

Therefore, the unconditional variance of  $\tilde{F}(\pi(\mathcal{D}_n))$  is

$$\begin{aligned}
\text{var}(\text{Top}_n(\pi(\mathcal{D}_n))) &= E \left( \text{var} \left( \text{Top}_n(\pi(\mathcal{D}_n)) \middle| \kappa(\pi) = k \right) \right) + \text{var} \left( E \left( \text{Top}_n(\pi(\mathcal{D}_n)) \middle| \kappa(\pi) = k \right) \right) \\
&= 2\sigma_1^2 - 4\sigma_2^2 + o(1).
\end{aligned} \tag{S.44}$$

In summary, we have

$$E(\text{Top}_n(\pi(\mathcal{D}_n))) = \mu_{\text{within}} + o(1), \quad \text{var}(\text{Top}_n(\pi(\mathcal{D}_n))) = 2\sigma_1^2 - 4\sigma_2^2 + o(1). \tag{S.45}$$

Compare Equation (S.45) with (S.19), we see that except for a small  $o(1)$  error term, the permuted  $\text{Top}_n$  has the same mean and variance as its theoretical counterparts under  $H_0$  (without permutation). Due to Theorem S2, we know that we can make the same conclusion for the  $F$ -statistics: the permutation-based null distribution of the distance-based  $F$ -statistic is asymptotically equivalent to its theoretical null distribution up to the first and second order moments, which is stated in the following Equation

$$\lim_{n \rightarrow \infty} E(F(\pi(\mathcal{D}_n))) = 1, \quad \lim_{n \rightarrow \infty} \text{var}(F(\pi(\mathcal{D}_n))) = \frac{2\sigma_1^2 - 4\sigma_2^2}{\mu_{\text{within}}^2}. \tag{S.46}$$

The above Equation completes the second half of Theorem 2 in the main text. Given the fact that there is no universal asymptotic distribution of these  $F$ -statistics, being able to show that the first and second order moments of  $F(\pi(\mathcal{D}_n))$  under both  $H_0$  and  $H_1$  match those of  $F(\mathcal{D}_n)$  under  $H_0$  is perhaps the best theoretical result we can hope for.

## S1.7 Squared Euclidean Distance of Multivariate Normal Random Vectors

In this section, we give detailed derivations of the results presented in Section 3.4 of the main text.

Let  $\mathcal{D}_{ij} := d^2(X_i, X_j)$  be the squared Euclidean distance between two  $p$ -dimensional random vectors  $X_i$  and  $X_j$  with the following multivariate normal distribution

$$X_i = Z_i + \mathbf{m}_i, \quad Z_i \sim N(0_v, I_v), \quad \mathbf{m}_i = \begin{cases} 0_v, & i \in A, \\ \mathbf{v}, & i \in B. \end{cases} \quad H_0 : \mathbf{v} = 0_v, \quad H_1 : \mathbf{v} \neq 0_v. \quad (\text{S.47})$$

In other words, all  $X_i$  share the identity covariance matrix. The mean vector of  $X_i$  in group  $A$  is the zero vector; the mean vector in group  $B$  ( $\mathbf{v}$ ) is a nonzero vector under  $H_1$ . Collectively, we can also use matrix notation to represent the data

$$X = Z + 1_B \mathbf{v}', \quad X, Z \in M_{n \times v}, \quad \text{vec}(Z) \sim N(0_{nv}, I_{nv}). \quad (\text{S.48})$$

By definition, we know that

$$\begin{aligned} \mathcal{D}_{ij} &= \sum_{l=1}^v (X_{il} - X_{jl})^2 = \sum_{l=1}^v (X_{il}^2 - 2X_{il}X_{jl} + X_{jl}^2). \\ E(X_{il}) &= \begin{cases} 0, & i \in A, \\ \mathbf{v}_l, & i \in B. \end{cases}, \quad E(X_{il}^2) = \begin{cases} 1, & i \in A, \\ 1 + \mathbf{v}_l^2, & i \in B. \end{cases} \end{aligned}$$

Therefore

$$E(\mathcal{D}_{ij}) = \begin{cases} 0, & i = j. \\ \mu_{\text{within}} = 2v, & i, j \in A \text{ or } i, j \in B, i \neq j. \\ \mu_{\text{between}} = 2v + \delta_\mu, & i \in A, j \in B, \text{ or } i \in B, j \in A. \end{cases}, \quad \delta_\mu := \|\mathbf{v}\|^2. \quad (\text{S.49})$$

### S1.7.1 Covariance of Squared Euclidean Distance

As we pointed out earlier, depending on the set of indices  $(i, j, i', j')$ ,  $\Sigma_{i,j,i',j'}$  can take four different **nonzero** values, which are  $\sigma_1^2, \sigma_2^2, \sigma_4^2$ , and  $\sigma_4^2$  listed in Section S1.1. We will compute these covariances as follows.

By construction, we know that  $(X_{ik} - X_{jk})^2$ , which are the building block of  $\mathcal{D}_{ij}$ , follows a scaled central  $\chi^2$ -distribution if  $i$  and  $j$  are from the same group (denoted by  $i \sim j$ ), or a noncentral  $\chi^2$ -distribution when  $i$  and  $j$  are from different groups (denoted by  $i \not\sim j$ ).

$$\begin{aligned} (X_{ik} - X_{jk})^2 &\sim 2Q, \quad Q \sim \begin{cases} \chi_1^2, & i \sim j. \\ \chi_1^2(\mathbf{v}_k^2/2), & i \not\sim j. \end{cases} \\ E((X_{ik} - X_{jk})^2) &= \begin{cases} 2, & i \sim j. \\ 2 + \mathbf{v}_k^2, & i \not\sim j. \end{cases}, \quad \text{var}((X_{ik} - X_{jk})^2) = \begin{cases} 8, & i \sim j. \\ 8 + 8\mathbf{v}_k^2, & i \not\sim j. \end{cases} \end{aligned}$$

With more derivations, we know that

$$\begin{aligned}\text{cov}(X_{ik}^2, X_{ik}X_{jk}) &= E(X_{ik}^3)E(X_{jk}) - E(X_{ik}^2)E(X_{ik})E(X_{jk}) = \begin{cases} 2\mathbf{v}_k^2, & i, j \in B \\ 0, & \text{otherwise.} \end{cases} \\ \text{cov}(X_{ik}X_{jk}, X_{ik}X_{j'k}) &= E(X_{ik}^2)E(X_{jk})E(X_{j'k}) - (E(X_{ik}))^2E(X_{jk})E(X_{j'k}) = E(X_{jk})E(X_{j'k}) \\ &= \begin{cases} \mathbf{v}_k^2, & j, j' \in B \\ 0, & \text{otherwise.} \end{cases}\end{aligned}$$

Assuming that  $i \in A$ , we have

$$\begin{aligned}\text{cov}((X_{ik} - X_{jk})^2, (X_{ik} - X_{j'k})^2) &= \text{var}(X_{ik}^2) - 2\text{cov}(X_{ik}^2, X_{ik}X_{jk}) - 2\text{cov}(X_{ik}^2, X_{ik}X_{j'k}) \\ &\quad + 4\text{cov}(X_{ik}X_{jk}, X_{ik}X_{j'k}) \\ &= \begin{cases} 2 + 4\mathbf{v}_k^2, & j, j' \in B, \\ 2, & \text{otherwise.} \end{cases}\end{aligned}\tag{S.50}$$

Furthermore, we know that for all cases,  $(X_{ik} - X_{jk})^2$  is independent of  $(X_{i'k} - X_{j'k})^2$  for  $k \neq k'$ , therefore

$$\begin{aligned}\text{cov}(\mathcal{D}_{ij}, \mathcal{D}_{i'j'}) &= \sum_{k=1}^v \sum_{k'=1}^v \text{cov}((X_{ik} - X_{jk})^2, (X_{i'k'} - X_{j'k'})^2) \\ &= \sum_{k=1}^v \text{cov}((X_{ik} - X_{jk})^2, (X_{i'k} - X_{j'k})^2).\end{aligned}\tag{S.51}$$

With the above derivations, we conclude that

Case 1:  $AAAA$  or  $BBBB$ ;  $i = i', j = j'$ , or  $i = j', i' = j$ .

$$\sigma_1^2 = E(\mathcal{D}_{ij}^2) = \sum_{k=1}^v \text{var}((X_{ik} - X_{jk})^2) = 8v.\tag{S.52}$$

Case 2 and 3:  $AAAA$  or  $BBBB$ ;  $(i = i', j \neq j')$ ,  $(i = j', i' \neq j)$ ,  $(i \neq j', j = i')$ , or  $(i \neq i', j = j')$ ;  $(AAB, i = i' \text{ or } j = i')$ ,  $(AABA, i = j' \text{ or } j = j')$ ,  $(ABAA, i = i' \text{ or } i = j')$ ,  $(BAAA, j = i' \text{ or } j = j')$ .

$$\sigma_2^2 = \sigma_3^2 = \sum_{k=1}^v \text{cov}((X_{ik} - X_{jk})^2, (X_{ik} - X_{j'k})^2) = 2v.\tag{S.53}$$

Case 4:  $(ABAB, i = i', j = j')$ ,  $(ABBA, i = j', j = i')$ ,  $(BAAB, i = j', j = i')$ ,  $(BABA, i = i', j = j')$ .

$$\sigma_4^2 = \sum_{k=1}^v \text{var}((X_{ik} - X_{jk})^2) = 8v + 8\|\mathbf{v}\|^2.\tag{S.54}$$

Case 5:  $(ABAB, i = i', j \neq j' \text{ or } i \neq i', j = j')$ ,  $(ABBA, i = j', j \neq i' \text{ or } i \neq j', j = i')$ ,  $(BAAB, i = j', j \neq i' \text{ or } i \neq j', j = i')$ ,  $(BABA, i = i', j \neq j' \text{ or } i \neq i', j = j')$ .

$$\sigma_5^2 = \sum_{k=1}^v \text{cov}((X_{ik} - X_{jk})^2, (X_{ik} - X_{j'k})^2) = 2v + 4\|\mathbf{v}\|^2.\tag{S.55}$$

Table S1: Classifying nonzero entries in  $\Sigma$ , the covariance matrix of the Euclidean squared distance matrix. Due to the assumption of group-symmetry, we only list one representative group membership in each case (e.g., AAAA represents both AAAA and BBBB). Note that the mathematical expectations of within-group and between-group distances are  $\mu_{\text{within}} = 2v$  and  $\mu_{\text{between}} = 2v + \|\mathbf{v}\|^2$ , respectively.

| Cases                             | $E(\mathcal{D}_{ij})$   | $E(\mathcal{D}_{i'j'})$ | $\Sigma_{i,j,i',j'}$                  | Size                                                     |
|-----------------------------------|-------------------------|-------------------------|---------------------------------------|----------------------------------------------------------|
| Case 1: AAAA, $i = i', j = j'$    | $2v$                    | $2v$                    | $\sigma_1^2 = 8v$                     | $m_1 = 2(n_A(n_A - 1) + n_B(n_B - 1))$                   |
| Case 2: AAAA, $i = i', j \neq j'$ | $2v$                    | $2v$                    | $\sigma_2^2 = 2v$                     | $m_2 = 4(n_A(n_A - 1)(n_A - 2) + n_B(n_B - 1)(n_B - 2))$ |
| Case 3: AAAB, $i = i', j \neq j'$ | $2v$                    | $2v + \ \mathbf{v}\ ^2$ | $\sigma_2^2 = 2v$                     | $m_3 = 8n_A n_B (n - 2)$                                 |
| Case 4: ABAB, $i = i', j = j'$    | $2v + \ \mathbf{v}\ ^2$ | $2v + \ \mathbf{v}\ ^2$ | $\sigma_3^2 = 8v + 8\ \mathbf{v}\ ^2$ | $m_4 = 4n_A n_B$                                         |
| Case 5: ABAB, $i = i', j \neq j'$ | $2v + \ \mathbf{v}\ ^2$ | $2v + \ \mathbf{v}\ ^2$ | $\sigma_4^2 = 2v + 4\ \mathbf{v}\ ^2$ | $m_5 = 4n_A n_B (n - 2)$                                 |

We list  $E(\mathcal{D}_{ij})$ ,  $E(\mathcal{D}_{i'j'})$ ,  $\Sigma_{i,j,i',j'}$ , and the size of each case in Table S1.

We conducted a small simulation study (SIM1) to show that the above theoretical derivations are correct. In each one of the 10,000 repetitions, we generated  $n_A = 3$  and  $n_B = 5$  random vector  $X_i$  in  $\mathbb{R}^4$  in this way

$$X_i \sim N(\mathbf{v}, I_4), \quad \begin{cases} \mathbf{v} = 0_4, & i \in A, \\ \mathbf{v} = (-1, 1/2, 2, 1)', & i \in B. \end{cases} \quad (\text{S.56})$$

We then computed  $\mathcal{D}$ , the Euclidean pairwise distance matrix, for each repetition. Finally, we estimated the mean and covariance of  $\mathcal{D}$  from all repetitions, and compared them with the theoretical results presented in Equations (S.49) and Table S1 in Figure S1. These figures validates theoretical derivations of the mean and covariance of  $\mathcal{D}$  summarized in Equation (S.49) and Table S1, and demonstrate the complexity of the covariance matrix of  $\mathcal{D}$ .

### S1.7.2 Mean and Variance of Total Squared Euclidean Distance

As a special case of Equations (S.12) and (S.13), for the squared Euclidean distance, we have

$$E(H_n) = \mu_{\text{within}}(n^2 - n) + 2\delta_\mu n_A n_B = 2v(n^2 - n) + 2\|\mathbf{v}\|^2 n_A n_B. \quad (\text{S.57})$$

$$\begin{aligned} \text{var}(H_n) &= (2(n_A^2 + n_B^2) - 2n)\sigma_1^2 + 4(n_A^3 + n_B^3 - 3(n_A^2 + n_B^2) + 2n + 2n_A n_B(n - 2))\sigma_2^2 \\ &\quad + 4n_A n_B \sigma_3^2 + 4n_A n_B (n - 2)\sigma_4^2 \\ &= 8vn^2(n - 1) + 16nn_A(n - n_A)\|\mathbf{v}\|^2. \end{aligned} \quad (\text{S.58})$$

Alternatively, we can derive the approximate variance of  $H_n$  with just the first two terms in Equation (S.13). Recall that in this case,  $\delta_{\sigma^2} := \sigma_4^2 - \sigma_2^2 = 4\|\mathbf{v}\|^2$ , therefore

$$\begin{aligned} \text{var}(H_n) &= \underbrace{4n^3\sigma_2^2}_{O(n^3)} + \underbrace{4nn_A n_B \delta_{\sigma^2}}_{O(n^{2.5})} + O(n^2) \\ &= 8vn^3 + 16nn_A n_B \|\mathbf{v}\|^2. \end{aligned} \quad (\text{S.59})$$

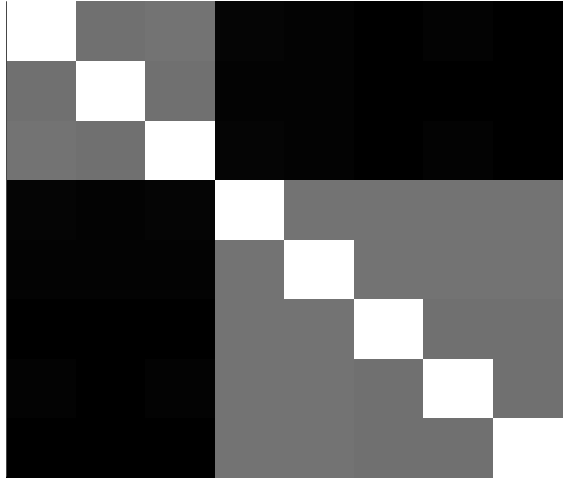

(A)

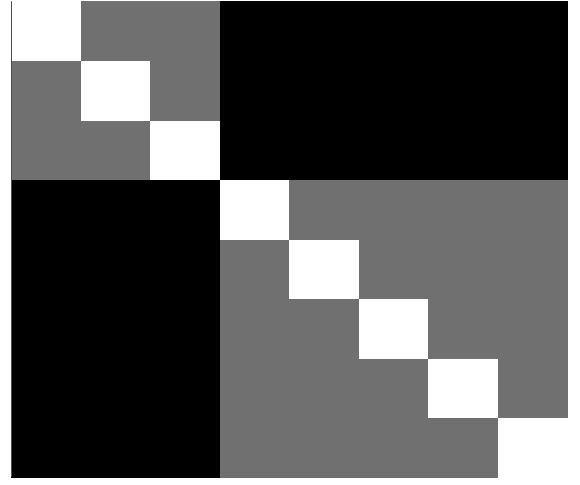

(B)

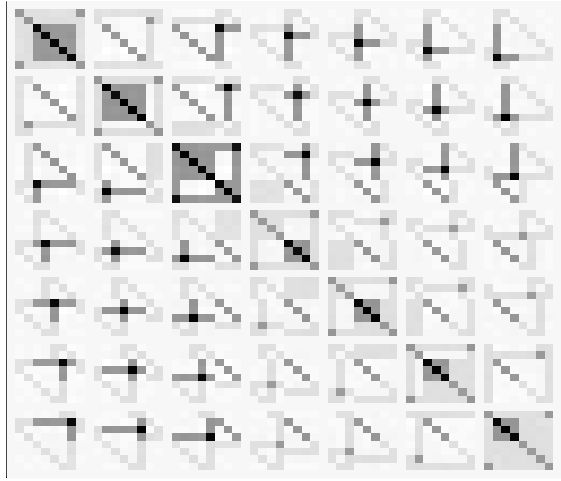

(C)

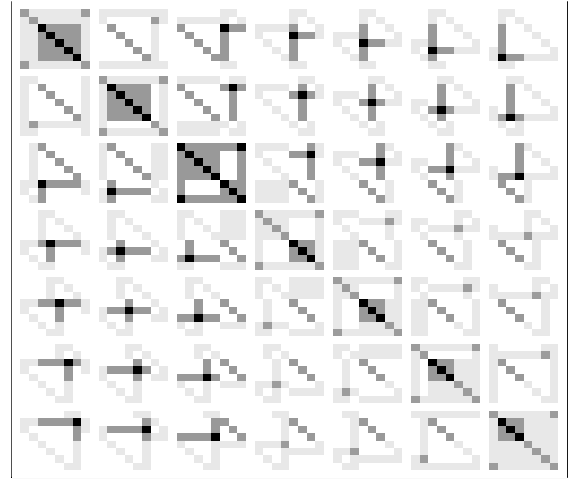

(D)

Figure S1: The mean and covariance of Euclidean pairwise distance matrix for SIM1. (A): Sample mean squared Euclidean distance,  $\bar{\mathcal{D}}$ , estimated from 10,000 simulations. (B): Theoretical  $E(\mathcal{D})$  computed by Equation (S.49). (C): Sample  $\hat{\Sigma}$  estimated from 10,000 simulations. (D): Theoretical  $\Sigma$  computed by Table S1.

By comparing Equations (S.59) and (S.58), we see that using just the first two terms in Equation (S.13) provides a very good large sample approximation of  $\text{var}(H_n)$  with the squared Euclidean distance.

### S1.7.3 Asymptotic Properties of $F(\mathcal{D})$ for Euclidean Distance

For squared Euclidean distance defined in Section S1.7, let  $S := XX'$  be the pairwise inner product of  $X$ ; let  $S_A$  and  $S_B$  be the submatrix of  $S$  that corresponds with samples in groups  $A$  and  $B$ , respectively. We have

$$\frac{H_n}{n} = \frac{1}{n} \sum_{i,i',l} (X_{il} - X_{i'l})^2 = 2\text{tr}(S) - \frac{2}{n} \sum_{l=1}^v \left( \sum_{i=1}^n X_{il} \right)^2. \quad (\text{S.60})$$

In this special case, we can greatly simplify  $\text{Top}_n$  by linear algebra techniques. First, let

$$P_{\text{Top}_n} := \frac{J_n}{n} - \frac{J_A}{n_A} - \frac{J_B}{n_B} = -\mathbf{v}\mathbf{v}', \quad \mathbf{v} := \sqrt{\frac{n_B}{n_A n}} \cdot \mathbf{1}_A - \sqrt{\frac{n_A}{n_B n}} \cdot \mathbf{1}_B, \quad \|\mathbf{v}\| = 1. \quad (\text{S.61})$$

By construction,  $P_{\text{Top}_n}$  is a *rank-one* matrix, and its only nonzero eigenvalue is  $\lambda = -1$ , with the corresponding eigenvector  $\mathbf{v}$ . Therefore

$$\begin{aligned} \text{Top}_n &= 2\text{tr}(S) - 2\text{tr}(S_A) - 2 - 2\text{tr}(S_B) \\ &\quad - \frac{2}{n} \sum_{l=1}^v \left( \sum_{i=1}^n X_{il} \right)^2 + \frac{2}{n_A} \sum_{l=1}^v \left( \sum_{i \in A} X_{il} \right)^2 + \frac{2}{n_B} \sum_{l=1}^v \left( \sum_{i \in B} X_{il} \right)^2 \\ &= -2 \sum_{l=1}^v X'_{\cdot l} \left( \frac{J_n}{n} - \frac{J_A}{n_A} - \frac{J_B}{n_B} \right) X_{\cdot l} = -2\text{tr}(X' P_{\text{Top}_n} X) \\ &:= 2 \sum_{l=1}^v \tilde{X}_l^2, \quad \tilde{X} := X' \mathbf{v} \in \mathbb{R}^v. \end{aligned} \quad (\text{S.62})$$

By construction,  $X = Z + \mathbf{1}_B \mathbf{v}'$ . Notice that  $\|\mathbf{v}\| = 1$  because it is an eigenvector. Let  $\tilde{Z} := Z' \mathbf{v} \in \mathbb{R}^v$ ,  $\tilde{Z} \sim N(0_v, I_v)$ , and

$$\tilde{X} = Z' \mathbf{v} + \mathbf{v} \mathbf{1}_B' \mathbf{v} = \tilde{Z} + \sqrt{\frac{n_A n_B}{n}} \mathbf{v} \sim N\left(\sqrt{\frac{n_A n_B}{n}} \mathbf{v}, I_v\right). \quad (\text{S.63})$$

Therefore

$$\text{Top}_n = 2 \sum_{l=1}^v \tilde{X}_l^2 \sim 2 \cdot \chi_v^2 \left( \frac{n_A n_B \delta_\mu}{n} \right). \quad (\text{S.64})$$

On the other hand, we know that

$$\frac{\text{Bottom}_n}{n-2} \sim AN\left(\mu_{\text{within}}, \frac{4\sigma_2^2}{n}\right) = AN\left(2v, \frac{8v}{n}\right). \quad (\text{S.65})$$

Therefore when  $n \rightarrow \infty$ ,

$$F \xrightarrow{d} \frac{1}{v} \cdot \chi_v^2 \left( \frac{n_A n_B \delta_\mu}{n} \right) = \frac{1}{v} \cdot \chi_v^2(c_\mu \lambda(1-\lambda)\sqrt{n}). \quad (\text{S.66})$$

Recall that in Section S1.5, we were only able to derive the asymptotic properties of the first and second moments of  $F(\mathcal{D})$ , which were summarized in Equation (S.27). By using the Euclidean distance, we can obtain

the asymptotic *distribution* of  $F(\mathcal{D})$  in addition to its mean and variance. On the other hand, Equation (S.66) also shows that, even for the Euclidean distance, the asymptotic distribution of  $F(\mathcal{D})$  still depends on  $v$ , which is a parameter of the underlying distribution of  $X$  (the “networks”). This fact shows that it is **impossible** to derive an universal asymptotic distribution of  $F(\mathcal{D})$  that works for all types of distance functions and the underlying distributions of the networks.

When a permutation  $\pi$  is applied to the data, we know that  $X$  will be replaced by  $\check{\pi}X$ , where  $\check{\pi} \in M_{n \times n}$  is the matrix representation of  $\pi$ .

Let  $\kappa(\pi) = k$ . It is easy to show that

$$\begin{aligned} 1'_A \check{\pi} 1_B &= n_A - k, & 1'_B \check{\pi} 1_B &= n_B - n_A + k. \\ \mathbf{v}' \check{\pi} X &= \mathbf{v}' \check{\pi} (Z + 1_B \mathbf{v}') \\ &= \mathbf{v}' \check{\pi} Z + \sqrt{\frac{n_B}{n_A n}} \cdot 1'_A \check{\pi} 1_B \mathbf{v}' - \sqrt{\frac{n_A}{n_B n}} \cdot 1'_B \check{\pi} 1_B \mathbf{v}' \\ &= \check{Z} + c_\pi \mathbf{v}'. \end{aligned}$$

$$\begin{aligned} \check{Z} &:= \mathbf{v}' \check{\pi} Z \sim N(0'_v, I_v), & c_\pi &:= \left( (n_A - k) \sqrt{\frac{n_B}{n_A n}} - (n_B - n_A + k) \sqrt{\frac{n_A}{n_B n}} \right). \\ c_\pi^2 &= \frac{(n_A - k)^2 n_B}{n_A n} + \frac{(n_B - n_A + k)^2 n_A}{n_B n} - \frac{2(n_A - k)(n_B - n_A + k)}{n} \\ &= \frac{(n_A^2 - nk)^2}{n_A n_B n}. \end{aligned}$$

Using the same technique employed in Equation (S.62), we can show the conditional distribution of  $\text{Top}_n(\pi(\mathcal{D}_n))$  follows the following noncentral  $\chi^2$  distribution.

$$\text{Top}_n(\pi(\mathcal{D}_n)) = -2\text{tr}(X' \check{\pi}' P_{\text{Top}_n} \check{\pi} X) = 2\|\mathbf{v}' \check{\pi} X\|^2 \sim 2 \cdot \chi_v^2(\lambda_\pi), \quad \lambda_\pi := c_\pi^2 \delta_\mu. \quad (\text{S.67})$$

Note that

$$\begin{aligned} E(c_\pi^2) &= \frac{n_A^4 - 2nn_A \cdot \frac{n_A^2}{n} + n_A^4 + \frac{n_A^2 n_B^2}{n} + O(n^2)}{nn_A n_B} = \frac{n_A n_B}{n^2} + O(n^{-1}) = O(1). \\ E(c_\pi^4) &= \frac{n_A^8 - 4n_A^6 n E(\kappa) + 6n_A^4 n^2 E(\kappa^2) - 4n_A^2 n^3 E(\kappa^3) + n^4 E(\kappa^4)}{n^2 n_A^2 n_B^2} \\ &= \frac{n_A^8 - 4n_A^8 + 6n_A^4 \left( n_A^4 + \frac{n_A^2 n_B^2}{n} \right) - 4n_A^2 \left( n_A^6 + \frac{3n_A^4 n_B^2}{n} \right) + n_A^8 + \frac{6n_A^6 n_B^2}{n} + O(n^6)}{n^2 n_A^2 n_B^2} \\ &= O(1). \end{aligned} \quad (\text{S.68})$$

Based on Assumption (3.15), we know that  $\delta_\mu = O(n^{-1/2})$ , thus  $\lambda_\pi$  converges to zero at the rate of  $O(n^{-1/2})$

$$E(\lambda_\pi) = O(n^{-1/2}), \quad \text{var}(\lambda_\pi) = O(n^{-1}). \quad (\text{S.69})$$

While not 100 percent rigorous, I think the following argument is convincing enough. If needed, we can do some more work (prove based on the conditional distribution and the definition of weak convergence) to make the following argument more rigorous.

Therefore, the distribution of  $\text{Top}_n(\pi(\mathcal{D}_n))$  given  $\kappa(\pi) = k$  converges in distribution to  $\chi_v^2$ , a centered  $\chi^2$ -distribution, irrespective of the value of  $k$ , hence its unconditional distribution must also be  $\chi_v^2$ . Using the fact that

the asymptotic distribution of  $\text{Top}_n(\pi(\mathcal{D}_n))$  and  $F(\pi(\mathcal{D}))$  are equivalent, we conclude that when  $n \rightarrow \infty$ ,

$$F(\pi(\mathcal{D})) \xrightarrow{d} \frac{1}{v} \cdot \chi_v^2. \quad (\text{S.70})$$

In other words, the permutation-based null distribution and the true null distribution of the  $F$ -statistic are asymptotically equivalent.

We conducted a second simulation study, SIM2, to validate the asymptotic distribution of  $F(\mathcal{D})$  and  $F(\pi(\mathcal{D}))$  presented in Equations (S.66) and (S.70). In each one of the 100,000 repetitions, we generated  $n_A = 100$  and  $n_B = 80$  independent random vectors  $X_{i\cdot}$  in  $\mathbb{R}^4$  in this way

$$X_{i\cdot} \sim N(\mathbf{v}, I_4), \quad \begin{cases} \mathbf{v} = 0_4, & i \in A, \\ \mathbf{v} = (\frac{1}{4}, \frac{1}{8}, \frac{1}{2}, \frac{1}{4})', & i \in B. \end{cases} \quad (\text{S.71})$$

We then computed  $\mathcal{D}$ , the Euclidean pairwise distance matrix, for each repetition. Based on these matrices, we calculate  $F(\mathcal{D})$  and their permuted counterparts,  $F(\pi(\mathcal{D}))$ . The histogram of  $F(\mathcal{D})$  and  $F(\pi(\mathcal{D}))$  calculated from these 100,000 repetitions, as well as their corresponding theoretical density curves represented in Equations (S.66) and (S.70), are shown in Figure S2. We see that the theoretical densities are good approximations of the empirical densities of  $F(\mathcal{D})$  and  $F(\pi(\mathcal{D}))$ . Specifically, the empirical densities of  $F(\pi(\mathcal{D}))$  (permuted  $F$ -statistics under  $H_1$ ) is equivalent to that of  $F(\mathcal{D})$  under  $H_0$ .

#### S1.7.4 Conclusions Based on the Euclidean Distance

In Section S1.6, we concluded that the unconditional mean and variance of  $\text{Top}_n(\pi(\mathcal{D}_n))$  is the same as its theoretical (unpermuted) mean and variance, but we were not able to prove that the distribution of  $F(\pi(\mathcal{D}_n))$  converges weakly to the theoretical distribution of the  $F$ -statistic under  $H_0$ , largely because there is no universal limiting distribution of  $F(\pi(\mathcal{D}_n))$  for all distances. In Section S1.7.3, we see that when the exact form of the distance is given, it is possible to obtain much stronger conclusions. Specifically, we were able to derive the limiting distribution of  $F(\pi(\mathcal{D}_n))$ , and prove that the theoretical and permutation-based null distributions of  $F$ -statistics are asymptotically equivalent.

Last but not the least, we would like to point out that, when the theoretical and permutation-based null distributions of  $F$ -statistics are asymptotically equivalent (as in the case of the Euclidean distance), the permutation test attains 100% asymptotic relative efficiency (ARE) compared with the **parametric test** based on the theoretical distribution of the  $F$ -statistic.

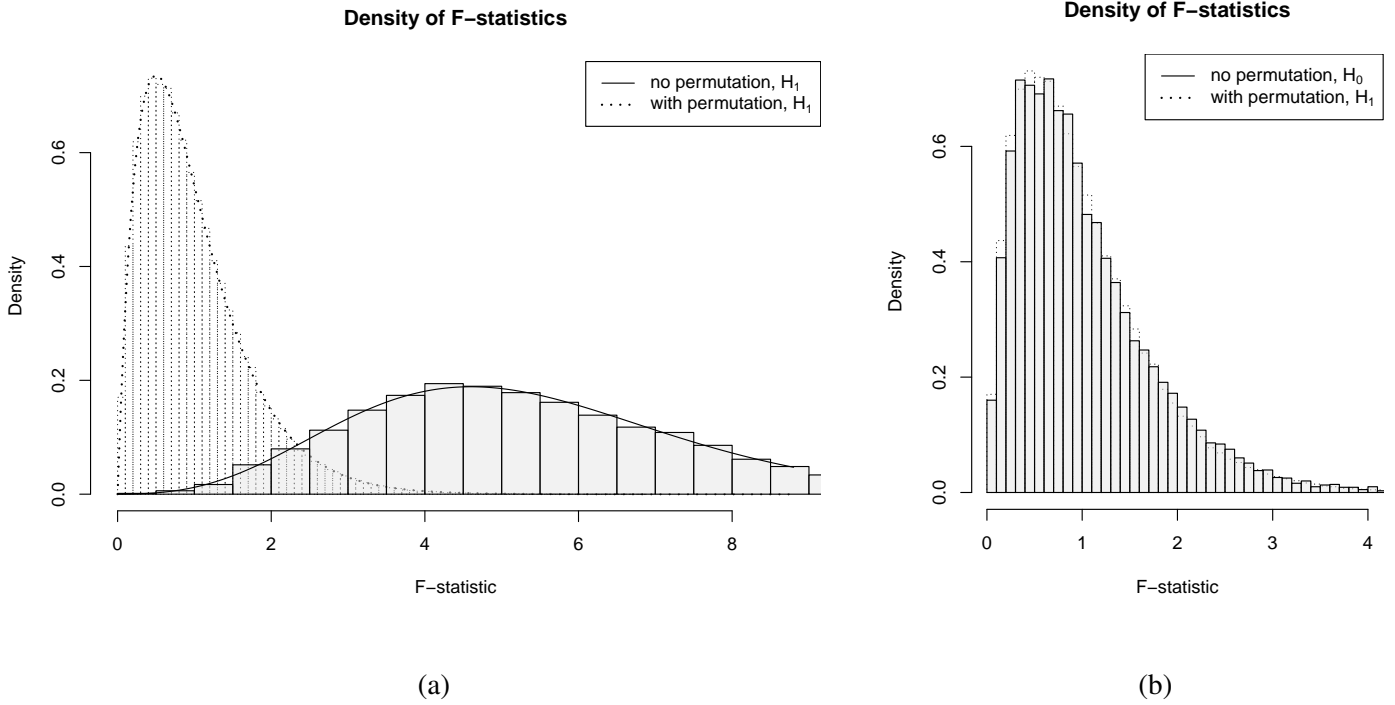

Figure S2: Comparing theoretical and empirical densities of  $F$ -statistics. Histograms represent empirical densities of  $F$ -statistics from 100,000 randomly generated data in SIM2. Solid bars represent densities of  $F$ -statistics without permutation ( $F(\mathcal{D})$ , either under  $H_0$  or  $H_1$ ), dotted bars represent empirical densities of  $F$ -statistics with random permutation ( $F(\pi(\mathcal{D}))$  under  $H_1$ ). (a) Densities of  $F$ -statistics with and without permutation under  $H_1$ . For comparison, theoretical densities are superimposed as the solid (no permutation, based on Equation (S.66)) and dotted curve (permuted, based on Equation (S.70)). (b) Comparing the empirical densities of permuted  $F$ -statistics under  $H_1$  (dotted bars) and the empirical densities of  $F$ -statistics under  $H_0$  without permutation (solid bars).

## S2 Additional Simulation Result

Table S2: Simulation Results of Experiment 1.a. in Scenario 1. Examine the power of discriminating ER and BP distributions under different edge densities. Based on 1000 iterations and calculating the rates of rejecting the null hypothesis under the 0.05 significance level. Two groups of unweighted graphs are generated from two distributions with Sample Size = 20, Vertex Size=20 and same edge densities.

| Experiment 1.a. Power for unweighted graph, ER vs BP |      |          |           |               |              |          |
|------------------------------------------------------|------|----------|-----------|---------------|--------------|----------|
| Edge                                                 | Den- | Proposed | Chen Test | Ginestet Test | Global effi- | Binomial |
| sity                                                 |      | Method   |           |               | ciency Test  | Test     |
| 0.02                                                 |      | 0.217    | 0.242     | 0.58          | 0.04         | 0.038    |
| 0.04                                                 |      | 0.21     | 0.156     | 0.291         | 0.048        | 0.042    |
| 0.06                                                 |      | 0.463    | 0.255     | 0.029         | 0.051        | 0.048    |
| 0.08                                                 |      | 0.722    | 0.395     | 0             | 0.044        | 0.034    |
| 0.1                                                  |      | 0.923    | 0.617     | 0             | 0.06         | 0.061    |
| 0.12                                                 |      | 0.995    | 0.776     | 0             | 0.047        | 0.052    |
| 0.14                                                 |      | 1        | 0.894     | 0             | 0.049        | 0.041    |
| 0.16                                                 |      | 1        | 0.962     | 0             | 0.051        | 0.051    |
| 0.18                                                 |      | 1        | 0.995     | 0             | 0.049        | 0.038    |
| 0.2                                                  |      | 1        | 1         | 0             | 0.056        | 0.046    |
| 0.22                                                 |      | 1        | 1         | 0             | 0.05         | 0.042    |
| 0.24                                                 |      | 1        | 1         | 0             | 0.052        | 0.048    |
| 0.26                                                 |      | 1        | 1         | 0             | 0.035        | 0.036    |
| 0.28                                                 |      | 1        | 1         | 0             | 0.052        | 0.037    |
| 0.3                                                  |      | 1        | 1         | 0             | 0.049        | 0.052    |

Table S3: Simulation Results of Experiment 1.b. in Scenario 1. Examine the power of discriminating ER and BA distributions under different edge densities. Based on 1000 iterations and calculating the rates of rejecting the null hypothesis under the 0.05 significance level. Two groups of unweighted graphs are generated from two distributions with Sample Size = 20, Vertex Size=20 and same edge densities.

| Experiment 1.b. Power for unweighted graph, ER vs BA |                    |           |               |                             |                  |  |
|------------------------------------------------------|--------------------|-----------|---------------|-----------------------------|------------------|--|
| Edge Den-<br>sity                                    | Proposed<br>Method | Chen Test | Ginestet Test | Global effi-<br>ciency Test | Binomial<br>Test |  |
| 0.05                                                 | 1                  | 1         | 0             | 1                           | 0.005            |  |
| 0.1                                                  | 1                  | 1         | 0             | 1                           | 0.004            |  |
| 0.14                                                 | 1                  | 1         | 0             | 1                           | 0.008            |  |
| 0.18                                                 | 1                  | 1         | 0             | 1                           | 0.006            |  |
| 0.22                                                 | 1                  | 1         | 0             | 1                           | 0.009            |  |
| 0.26                                                 | 1                  | 1         | 0             | 1                           | 0.001            |  |
| 0.29                                                 | 1                  | 1         | 0             | 1                           | 0.007            |  |
| 0.33                                                 | 1                  | 1         | 0             | 1                           | 0.005            |  |
| 0.36                                                 | 1                  | 1         | 0.01          | 1                           | 0.003            |  |
| 0.38                                                 | 1                  | 1         | 0.028         | 1                           | 0.006            |  |

Table S4: Simulation Results of Experiment 1.c. in Scenario 1. Examine the type 1 error of ER's under different edge densities. Based on 1000 iterations and calculating the rates of rejecting the null hypothesis under the 0.05 significance level. Two groups of unweighted graphs are generated from two distributions with Sample Size = 20, Vertex Size=20 and same edge densities.

| Experiment 1.c. Type 1 error for unweighted graph, ER vs ER |                    |           |               |                             |                  |  |
|-------------------------------------------------------------|--------------------|-----------|---------------|-----------------------------|------------------|--|
| Edge Den-<br>sity                                           | Proposed<br>Method | Chen Test | Ginestet Test | Global effi-<br>ciency Test | Binomial<br>Test |  |
| 0.1                                                         | 0.056              | 0.049     | 0             | 0.053                       | 0.058            |  |
| 0.3                                                         | 0.041              | 0.051     | 0             | 0.051                       | 0.055            |  |
| 0.5                                                         | 0.044              | 0.06      | 0             | 0.045                       | 0.051            |  |
| 0.7                                                         | 0.047              | 0.051     | 0             | 0.049                       | 0.057            |  |
| 0.9                                                         | 0.052              | 0.057     | 0             | 0.047                       | 0.046            |  |

Table S5: Simulation Results of Experiment 3.a. under Scenario 3. Examine both the power and type 1 error under the settings of  $\sigma^2=1$ ,  $\Sigma = I$  with full connection (edge density = 1). For one of the group, the average edge weight is fixed as  $\mu=10$  while for the other group the group mean edge weights vary from 8 to 12. Conducted based on 1000 iterations and calculating the rates of rejecting the null hypothesis under the 0.05 significance level. Two groups of graphs are generated from same distributions, ER, with Sample Size = 20 and Vertex Size=20. Experiment 3.a. Experiment 3.b. shares the same settings with 3.a. except for the covariance matrix  $\Sigma$  is set to be toeplitz( $1:\frac{1}{190}$ ) to introduce correlation between edge weights. Experiment 3.c. fixes  $\mu=4$ ,  $\sigma^2=0.25$ ,  $\Sigma = I$  for both groups while making changes in the edge densities. One group has its edge density equals to 0.5. The other group has its edge densities vary from 0.2 to 0.8.

| Experiment 3.a. Edge density=1; $\Sigma = I$ |                        |                    |           |                  |                             |
|----------------------------------------------|------------------------|--------------------|-----------|------------------|-----------------------------|
| Mean Group 1<br>(Edge)                       | Mean Group 2<br>(Edge) | Proposed<br>Method | Chen Test | Ginestet<br>Test | Global effi-<br>ciency Test |
| 10                                           | 8                      | 1                  | 1         | 0.983            | 1                           |
| 10                                           | 8.25                   | 1                  | 1         | 0.867            | 1                           |
| 10                                           | 8.5                    | 1                  | 1         | 0.499            | 1                           |
| 10                                           | 8.75                   | 1                  | 1         | 0.051            | 1                           |
| 10                                           | 9                      | 1                  | 1         | 0.002            | 1                           |
| 10                                           | 9.25                   | 1                  | 1         | 0                | 1                           |
| 10                                           | 9.5                    | 1                  | 1         | 0                | 1                           |
| 10                                           | 9.75                   | 1                  | 0.862     | 0                | 1                           |
| 10                                           | 10                     | 0.061              | 0.051     | 0                | 0.055                       |
| 10                                           | 10.25                  | 1                  | 0.871     | 0                | 1                           |
| 10                                           | 10.5                   | 1                  | 1         | 0                | 1                           |
| 10                                           | 10.75                  | 1                  | 1         | 0                | 1                           |
| 10                                           | 11                     | 1                  | 1         | 0                | 1                           |
| 10                                           | 11.25                  | 1                  | 1         | 0.049            | 1                           |
| 10                                           | 11.5                   | 1                  | 1         | 0.487            | 1                           |
| 10                                           | 11.75                  | 1                  | 1         | 0.89             | 1                           |
| 10                                           | 12                     | 1                  | 1         | 0.976            | 1                           |

Table S6: Simulation Results of Experiment 3.b. under Scenario 3. Examine both the power and type 1 error under the settings of  $\sigma^2=1$ ,  $\Sigma$  is set to be  $\text{toeplitz}(1:\frac{1}{190})$  with full connection (edge density = 1). For one of the group, the average edge weight is fixed as  $\mu=10$  while for the other group the group mean edge weights vary from 8 to 12. Conducted based on 1000 iterations and calculating the rates of rejecting the null hypothesis under the 0.05 significance level. Two groups of graphs are generated from same distributions, ER, with Sample Size = 20 and Vertex Size=20.

| Experiment 3.b. Edge density=1; $\Sigma=\text{toeplitz}(1:\frac{1}{190})$ |                        |                    |           |                  |                             |
|---------------------------------------------------------------------------|------------------------|--------------------|-----------|------------------|-----------------------------|
| Mean Group 1<br>(Edge)                                                    | Mean Group 2<br>(Edge) | Proposed<br>Method | Chen Test | Ginestet<br>Test | Global effi-<br>ciency Test |
| 10                                                                        | 8.5                    | 0.999              | 0.995     | 0.048            | 1                           |
| 10                                                                        | 8.65                   | 1                  | 0.963     | 0.017            | 1                           |
| 10                                                                        | 8.8                    | 0.99               | 0.905     | 0.006            | 0.991                       |
| 10                                                                        | 8.95                   | 0.973              | 0.793     | 0.002            | 0.967                       |
| 10                                                                        | 9.1                    | 0.911              | 0.657     | 0.001            | 0.906                       |
| 10                                                                        | 9.25                   | 0.809              | 0.501     | 0                | 0.804                       |
| 10                                                                        | 9.4                    | 0.607              | 0.326     | 0                | 0.61                        |
| 10                                                                        | 9.55                   | 0.364              | 0.17      | 0                | 0.355                       |
| 10                                                                        | 9.7                    | 0.175              | 0.072     | 0                | 0.184                       |
| 10                                                                        | 9.85                   | 0.1                | 0.045     | 0                | 0.09                        |
| 10                                                                        | 10                     | 0.039              | 0.055     | 0                | 0.039                       |
| 10                                                                        | 10.15                  | 0.082              | 0.06      | 0                | 0.08                        |
| 10                                                                        | 10.3                   | 0.223              | 0.113     | 0                | 0.205                       |
| 10                                                                        | 10.45                  | 0.399              | 0.179     | 0                | 0.375                       |
| 10                                                                        | 10.6                   | 0.618              | 0.315     | 0                | 0.6                         |
| 10                                                                        | 10.75                  | 0.812              | 0.467     | 0                | 0.793                       |
| 10                                                                        | 10.9                   | 0.93               | 0.639     | 0.001            | 0.902                       |
| 10                                                                        | 11.05                  | 0.976              | 0.817     | 0.007            | 0.972                       |
| 10                                                                        | 11.2                   | 0.992              | 0.899     | 0.01             | 0.992                       |
| 10                                                                        | 11.35                  | 0.999              | 0.973     | 0.021            | 1                           |
| 10                                                                        | 11.5                   | 1                  | 0.975     | 0.056            | 1                           |

Table S7: Simulation Results of Experiment 3.c. under Scenario 3. Examine both the power and type 1 error under the settings of  $\mu=4$ ,  $\sigma^2=0.25$ ,  $\Sigma = I$  for both groups. For one of the group, the edge density is fixed as 0.5 while for the other group has its edge densities vary from 0.3 to 0.7. Conducted based on 1000 iterations and calculating the rates of rejecting the null hypothesis under the 0.05 significance level. Two groups of graphs are generated from same distributions, ER, with Sample Size = 20 and Vertex Size=20.

| Experiment 3.c. Edge density=0.5; $\Sigma = I$ |                      |                 |           |               |                        |
|------------------------------------------------|----------------------|-----------------|-----------|---------------|------------------------|
| Edge Density Group 1                           | Edge Density Group 2 | Proposed Method | Chen Test | Ginestet Test | Global efficiency Test |
| 0.5                                            | 0.3                  | 1               | 1         | 0             | 1                      |
| 0.5                                            | 0.325                | 1               | 1         | 0             | 1                      |
| 0.5                                            | 0.35                 | 1               | 1         | 0             | 1                      |
| 0.5                                            | 0.375                | 1               | 1         | 0             | 1                      |
| 0.5                                            | 0.4                  | 1               | 0.998     | 0             | 1                      |
| 0.5                                            | 0.425                | 1               | 0.92      | 0             | 1                      |
| 0.5                                            | 0.45                 | 0.904           | 0.426     | 0             | 0.938                  |
| 0.5                                            | 0.475                | 0.341           | 0.111     | 0             | 0.422                  |
| 0.5                                            | 0.5                  | 0.054           | 0.054     | 0             | 0.043                  |
| 0.5                                            | 0.525                | 0.336           | 0.072     | 0             | 0.411                  |
| 0.5                                            | 0.55                 | 0.91            | 0.126     | 0             | 0.938                  |
| 0.5                                            | 0.575                | 0.996           | 0.338     | 0             | 0.999                  |
| 0.5                                            | 0.6                  | 1               | 0.734     | 0             | 1                      |
| 0.5                                            | 0.625                | 1               | 0.983     | 0             | 1                      |
| 0.5                                            | 0.65                 | 1               | 1         | 0             | 1                      |
| 0.5                                            | 0.675                | 1               | 1         | 0             | 1                      |
| 0.5                                            | 0.7                  | 1               | 1         | 0             | 1                      |

Table S8: Simulation Results of Highdimensional Case. BP vs ER; Power obtained from 500 repetition; Sample Size= 20; Vertex Size = 1000

| Edge Density | Highdimensional Ex-tension | Original Version |
|--------------|----------------------------|------------------|
| 0.05         | 1.000                      | 0.05             |
| 0.1          | 1.000                      | 1.000            |
